# Supplementary material for: Exact solution for the force-extension relation of a semiflexible polymer under compression
Source: arXiv:1705.03267 source file (2017-05-09)
Supplement: Supplementary file 1 [file Supplemental_Material_Kurzthaler.pdf]

# (A) Force-extension relation of compressed semiflexible polymers with different boundary conditions

## (A.1) Force-extension relation of a clamped semiflexible polymer with different persistence lengths $l_P$ and forces F

| | persistence length $l_P/L$ | | | | | | | | | | | | | | | | | | | |
|---|---|---|---|---|---|---|---|---|---|---|---|---|---|---|---|---|---|---|---|---|
| **$\|F\|/F_c$** | **0.1** | **0.2** | **0.3** | **0.4** | **0.5** | **0.6** | **0.7** | **0.8** | **0.9** | **1.0** | **1.5** | **2.0** | **3.0** | **4.0** | **5.0** | **6.0** | **7.0** | **8.0** | **9.0** | **10.0** |
| **0.00** | 0.1999 | 0.3929 | 0.5467 | 0.6495 | 0.7155 | 0.7597 | 0.7912 | 0.8150 | 0.8336 | 0.8488 | 0.8960 | 0.9207 | 0.9463 | 0.9594 | 0.9673 | 0.9727 | 0.9765 | 0.9794 | 0.9817 | 0.9835 |
| **0.05** | 0.1981 | 0.3879 | 0.5403 | 0.6432 | 0.7098 | 0.7546 | 0.7866 | 0.8107 | 0.8296 | 0.8450 | 0.8931 | 0.9184 | 0.9446 | 0.9581 | 0.9663 | 0.9718 | 0.9758 | 0.9787 | 0.9811 | 0.9829 |
| **0.10** | 0.1962 | 0.3830 | 0.5337 | 0.6366 | 0.7039 | 0.7492 | 0.7817 | 0.8061 | 0.8254 | 0.8411 | 0.8900 | 0.9159 | 0.9428 | 0.9567 | 0.9651 | 0.9708 | 0.9749 | 0.9780 | 0.9804 | 0.9823 |
| **0.15** | 0.1944 | 0.3779 | 0.5270 | 0.6299 | 0.6976 | 0.7436 | 0.7765 | 0.8013 | 0.8209 | 0.8368 | 0.8867 | 0.9132 | 0.9408 | 0.9551 | 0.9639 | 0.9697 | 0.9740 | 0.9772 | 0.9797 | 0.9817 |
| **0.20** | 0.1925 | 0.3729 | 0.5202 | 0.6229 | 0.6911 | 0.7376 | 0.7710 | 0.7962 | 0.8161 | 0.8323 | 0.8831 | 0.9103 | 0.9387 | 0.9534 | 0.9625 | 0.9686 | 0.9729 | 0.9763 | 0.9789 | 0.9809 |
| **0.25** | 0.1907 | 0.3678 | 0.5132 | 0.6156 | 0.6843 | 0.7313 | 0.7652 | 0.7908 | 0.8110 | 0.8275 | 0.8793 | 0.9071 | 0.9363 | 0.9516 | 0.9609 | 0.9672 | 0.9718 | 0.9752 | 0.9779 | 0.9801 |
| **0.30** | 0.1888 | 0.3627 | 0.5061 | 0.6081 | 0.6772 | 0.7247 | 0.7591 | 0.7851 | 0.8056 | 0.8223 | 0.8751 | 0.9036 | 0.9337 | 0.9495 | 0.9592 | 0.9658 | 0.9705 | 0.9741 | 0.9769 | 0.9792 |
| **0.35** | 0.1869 | 0.3576 | 0.4989 | 0.6004 | 0.6697 | 0.7178 | 0.7526 | 0.7789 | 0.7998 | 0.8168 | 0.8706 | 0.8997 | 0.9308 | 0.9472 | 0.9572 | 0.9641 | 0.9691 | 0.9728 | 1.0107 | 0.9781 |
| **0.40** | 0.1851 | 0.3524 | 0.4915 | 0.5924 | 0.6619 | 0.7105 | 0.7457 | 0.7724 | 0.7936 | 0.8108 | 0.8656 | 0.8955 | 0.9276 | 0.9445 | 0.9551 | 0.9622 | 0.9674 | 0.9713 | 0.9744 | 0.9769 |
| **0.45** | 0.1832 | 0.3472 | 0.4840 | 0.5842 | 0.6538 | 0.7028 | 0.7384 | 0.7655 | 0.7869 | 0.8045 | 0.8603 | 0.8909 | 0.9240 | 0.9416 | 0.9526 | 0.9601 | 0.9655 | 0.9696 | 0.9729 | 0.9755 |
| **0.50** | 0.1814 | 0.3419 | 0.4763 | 0.5756 | 0.6454 | 0.6946 | 0.7307 | 0.7581 | 0.7799 | 0.7976 | 0.8544 | 0.8857 | 0.9199 | 0.9382 | 0.9497 | 0.9576 | 0.9633 | 0.9677 | 0.9711 | 0.9739 |
| **0.55** | 0.1795 | 0.3366 | 0.4685 | 0.5669 | 0.6365 | 0.6861 | 0.7225 | 0.7502 | 0.7722 | 0.7902 | 0.8479 | 0.8800 | 0.9153 | 0.9344 | 0.9464 | 0.9547 | 0.9607 | 0.9654 | 0.9690 | 0.9720 |
| **0.60** | 0.1776 | 0.3313 | 0.4606 | 0.5578 | 0.6273 | 0.6771 | 0.7138 | 0.7418 | 0.7641 | 0.7823 | 0.8408 | 0.8736 | 0.9100 | 0.9299 | 0.9425 | 0.9513 | 0.9577 | 0.9626 | 0.9681 | 0.9701 |
| **0.65** | 0.1758 | 0.3260 | 0.4526 | 0.5485 | 0.6177 | 0.6676 | 0.7045 | 0.7329 | 0.7553 | 0.7738 | 0.8330 | 0.8665 | 0.9040 | 0.9247 | 0.9380 | 0.9472 | 0.9541 | 0.9593 | 0.9635 | 0.9668 |
| **0.70** | 0.1739 | 0.3206 | 0.4444 | 0.5389 | 0.6077 | 0.6576 | 0.6948 | 0.7233 | 0.7460 | 0.7645 | 0.8244 | 0.8585 | 0.8971 | 0.9187 | 0.9326 | 0.9424 | 0.9496 | 0.9553 | 0.9597 | 0.9634 |
| **0.75** | 0.1720 | 0.3152 | 0.4361 | 0.5290 | 0.5972 | 0.6471 | 0.6844 | 0.7131 | 0.7359 | 0.7546 | 0.8149 | 0.8495 | 0.8890 | 0.9115 | 0.9261 | 0.9365 | 0.9442 | 0.9507 | 0.9551 | 0.9590 |
| **0.80** | 0.1702 | 0.3098 | 0.4277 | 0.5189 | 0.5864 | 0.6361 | 0.6734 | 0.7022 | 0.7251 | 0.7438 | 0.8044 | 0.8393 | 0.8797 | 0.9029 | 0.9182 | 0.9292 | 0.9374 | 0.9439 | 0.9491 | 0.9534 |
| **0.85** | 0.1683 | 0.3044 | 0.4191 | 0.5085 | 0.5751 | 0.6245 | 0.6617 | 0.6905 | 0.7135 | 0.7322 | 0.7929 | 0.8278 | 0.8688 | 0.8926 | 0.9086 | 0.9201 | 0.9288 | 0.9359 | 0.9414 | 0.9460 |
| **0.90** | 0.1664 | 0.2989 | 0.4105 | 0.4978 | 0.5634 | 0.6124 | 0.6494 | 0.6781 | 0.7010 | 0.7197 | 0.7800 | 0.8149 | 0.8560 | 0.8802 | 0.8966 | 0.9086 | 0.9177 | 0.9251 | 0.9311 | 0.9361 |
| **0.95** | 0.1645 | 0.2934 | 0.4017 | 0.4869 | 0.5513 | 0.5996 | 0.6364 | 0.6649 | 0.6876 | 0.7062 | 0.7659 | 0.8002 | 0.8409 | 0.8652 | 0.8817 | 0.8939 | 0.9033 | 0.9109 | 0.9171 | 0.9224 |
| **1.00** | 0.1627 | 0.2879 | 0.3928 | 0.4757 | 0.5387 | 0.5863 | 0.6226 | 0.6508 | 0.6733 | 0.6917 | 0.7502 | 0.7836 | 0.8232 | 0.8469 | 0.8631 | 0.8750 | 0.8843 | 0.8918 | 0.8980 | 0.9033 |
| **1.05** | 0.1608 | 0.2824 | 0.3838 | 0.4642 | 0.5257 | 0.5724 | 0.6081 | 0.6359 | 0.6580 | 0.6761 | 0.7329 | 0.7650 | 0.8025 | 0.8247 | 0.8398 | 0.8512 | 0.8594 | 0.8662 | 0.8718 | 0.8764 |
| **1.10** | 0.1589 | 0.2768 | 0.3747 | 0.4525 | 0.5123 | 0.5578 | 0.5928 | 0.6201 | 0.6417 | 0.6593 | 0.7140 | 0.7440 | 0.7783 | 0.7980 | 0.8110 | 0.8201 | 0.8269 | 0.8321 | 0.8362 | 0.8395 |
| **1.15** | 0.1570 | 0.2712 | 0.3656 | 0.4406 | 0.4984 | 0.5427 | 0.5768 | 0.6033 | 0.6243 | 0.6413 | 0.6932 | 0.7205 | 0.7503 | 0.7662 | 0.7758 | 0.7819 | 0.7859 | 0.7885 | 0.7900 | 0.7909 |
| **1.20** | 0.1552 | 0.2657 | 0.3563 | 0.4284 | 0.4842 | 0.5270 | 0.5599 | 0.5856 | 0.6059 | 0.6221 | 0.6705 | 0.6945 | 0.7183 | 0.7291 | 0.7342 | 0.7361 | 0.7363 | 0.7354 | 0.7338 | 0.7318 |
| **1.25** | 0.1533 | 0.2601 | 0.3470 | 0.4160 | 0.4695 | 0.5107 | 0.5423 | 0.5670 | 0.5863 | 0.6017 | 0.6459 | 0.6658 | 0.6823 | 0.6869 | 0.6865 | 0.6837 | 0.6799 | 0.6755 | 0.6710 | 0.6666 |
| **1.30** | 0.1514 | 0.2545 | 0.3375 | 0.4034 | 0.4545 | 0.4938 | 0.5240 | 0.5474 | 0.5656 | 0.5800 | 0.6193 | 0.6346 | 0.6427 | 0.6403 | 0.6343 | 0.6271 | 0.6198 | 0.6130 | 0.6068 | 0.6014 |
| **1.35** | 0.1495 | 0.2488 | 0.3281 | 0.3906 | 0.4391 | 0.4764 | 0.5049 | 0.5269 | 0.5439 | 0.5571 | 0.5910 | 0.6010 | 0.6000 | 0.5907 | 0.5798 | 0.5693 | 0.5601 | 0.5522 | 0.5457 | 0.5403 |
| **1.40** | 0.1477 | 0.2432 | 0.3185 | 0.3777 | 0.4234 | 0.4584 | 0.4852 | 0.5056 | 0.5212 | 0.5331 | 0.5609 | 0.5653 | 0.5552 | 0.5398 | 0.5253 | 0.5132 | 0.5034 | 0.4958 | 0.4898 | 0.4851 |
| **1.45** | 0.1458 | 0.2376 | 0.3089 | 0.3646 | 0.4074 | 0.4400 | 0.4647 | 0.4834 | 0.4974 | 0.5079 | 0.5292 | 0.5280 | 0.5094 | 0.4894 | 0.4730 | 0.4606 | 0.4513 | 0.4445 | 0.4393 | 0.4353 |

| | | | | | | | | | | | | | | | | | | | | |
|---|---|---|---|---|---|---|---|---|---|---|---|---|---|---|---|---|---|---|---|---|
| **1.50** | 0.1439 | 0.2319 | 0.2992 | 0.3513 | 0.3911 | 0.4211 | 0.4437 | 0.4605 | 0.4728 | 0.4817 | 0.4963 | 0.4895 | 0.4637 | 0.4408 | 0.4240 | 0.4122 | 0.4040 | 0.3980 | 0.3936 | 0.3902 |
| **1.55** | 0.1420 | 0.2263 | 0.2895 | 0.3379 | 0.3745 | 0.4019 | 0.4221 | 0.4369 | 0.4474 | 0.4547 | 0.4625 | 0.4505 | 0.4191 | 0.3949 | 0.3788 | 0.3682 | 0.3609 | 0.3557 | 0.3518 | 0.3489 |
| **1.60** | 0.1401 | 0.2206 | 0.2798 | 0.3244 | 0.3577 | 0.3823 | 0.4001 | 0.4128 | 0.4214 | 0.4269 | 0.4280 | 0.4116 | 0.3764 | 0.3524 | 0.3374 | 0.3279 | 0.3215 | 0.3169 | 0.3135 | 0.3108 |
| **1.65** | 0.1383 | 0.2149 | 0.2700 | 0.3108 | 0.3408 | 0.3624 | 0.3777 | 0.3881 | 0.3948 | 0.3986 | 0.3932 | 0.3732 | 0.3361 | 0.3130 | 0.2995 | 0.2910 | 0.2852 | 0.2811 | 0.2780 | 0.2756 |
| **1.70** | 0.1364 | 0.2093 | 0.2602 | 0.2972 | 0.3237 | 0.3423 | 0.3550 | 0.3631 | 0.3678 | 0.3699 | 0.3586 | 0.3358 | 0.2983 | 0.2768 | 0.2645 | 0.2569 | 0.2517 | 0.2479 | 0.2450 | 0.2428 |
| **1.75** | 0.1345 | 0.2036 | 0.2504 | 0.2835 | 0.3065 | 0.3221 | 0.3321 | 0.3379 | 0.3406 | 0.3410 | 0.3244 | 0.2999 | 0.2632 | 0.2434 | 0.2323 | 0.2253 | 0.2205 | 0.2170 | 0.2143 | 0.2122 |
| **1.80** | 0.1326 | 0.1979 | 0.2406 | 0.2697 | 0.2892 | 0.3017 | 0.3091 | 0.3126 | 0.3134 | 0.3121 | 0.2909 | 0.2655 | 0.2306 | 0.2125 | 0.2023 | 0.1958 | 0.1913 | 0.1881 | 0.1856 | 0.1836 |
| **1.85** | 0.1307 | 0.1923 | 0.2308 | 0.2560 | 0.2720 | 0.2813 | 0.2860 | 0.2874 | 0.2862 | 0.2834 | 0.2585 | 0.2330 | 0.2003 | 0.1837 | 0.1743 | 0.1683 | 0.1641 | 0.1610 | 0.1586 | 0.1567 |
| **1.90** | 0.1289 | 0.1866 | 0.2210 | 0.2423 | 0.2547 | 0.2610 | 0.2631 | 0.2622 | 0.2594 | 0.2551 | 0.2272 | 0.2023 | 0.1721 | 0.1568 | 0.1481 | 0.1424 | 0.1385 | 0.1355 | 0.1333 | 0.1315 |
| **1.95** | 0.1270 | 0.1809 | 0.2112 | 0.2286 | 0.2375 | 0.2408 | 0.2403 | 0.2374 | 0.2329 | 0.2274 | 0.1972 | 0.1733 | 0.1457 | 0.1317 | 0.1235 | 0.1181 | 0.1144 | 0.1116 | 0.1094 | 0.1077 |
| **2.00** | 0.1251 | 0.1753 | 0.2014 | 0.2149 | 0.2204 | 0.2207 | 0.2178 | 0.2129 | 0.2069 | 0.2003 | 0.1687 | 0.1461 | 0.1210 | 0.1081 | 0.1003 | 0.0952 | 0.0916 | 0.0890 | 0.0869 | 0.0853 |
| **2.05** | 0.1232 | 0.1696 | 0.1917 | 0.2013 | 0.2034 | 0.2009 | 0.1957 | 0.1890 | 0.1816 | 0.1741 | 0.1416 | 0.1205 | 0.0977 | 0.0858 | 0.0785 | 0.0736 | 0.0702 | 0.0676 | 0.0656 | 0.0641 |
| **2.10** | 0.1213 | 0.1640 | 0.1820 | 0.1878 | 0.1866 | 0.1814 | 0.1740 | 0.1656 | 0.1571 | 0.1487 | 0.1159 | 0.0964 | 0.0758 | 0.0648 | 0.0578 | 0.0532 | 0.0499 | 0.0474 | 0.0455 | 0.0440 |
| **2.15** | 0.1195 | 0.1584 | 0.1723 | 0.1745 | 0.1700 | 0.1622 | 0.1528 | 0.1429 | 0.1333 | 0.1244 | 0.0917 | 0.0737 | 0.0551 | 0.0448 | 0.0383 | 0.0338 | 0.0306 | 0.0282 | 0.0264 | 0.0249 |
| **2.20** | 0.1176 | 0.1527 | 0.1627 | 0.1612 | 0.1537 | 0.1434 | 0.1321 | 0.1209 | 0.1105 | 0.1011 | 0.0688 | 0.0523 | 0.0355 | 0.0259 | 0.0197 | 0.0154 | 0.0124 | 0.0100 | 0.0083 | 0.0068 |
| **2.25** | 0.1157 | 0.1471 | 0.1532 | 0.1481 | 0.1376 | 0.1250 | 0.1120 | 0.0997 | 0.0886 | 0.0788 | 0.0472 | 0.0321 | 0.0169 | 0.0080 | 0.0021 | -0.0021 | -0.0050 | -0.0073 | -0.0090 | -0.0104 |
| **2.30** | 0.1138 | 0.1415 | 0.1437 | 0.1351 | 0.1218 | 0.1070 | 0.0926 | 0.0793 | 0.0676 | 0.0576 | 0.0268 | 0.0129 | -0.0009 | -0.0091 | -0.0147 | -0.0187 | -0.0216 | -0.0237 | -0.0254 | -0.0268 |
| **2.35** | 0.1119 | 0.1360 | 0.1342 | 0.1223 | 0.1063 | 0.0896 | 0.0738 | 0.0597 | 0.0476 | 0.0374 | 0.0075 | -0.0052 | -0.0178 | -0.0254 | -0.0308 | -0.0346 | -0.0373 | -0.0394 | -0.0411 | -0.0424 |
| **2.40** | 0.1101 | 0.1304 | 0.1249 | 0.1097 | 0.0911 | 0.0726 | 0.0557 | 0.0409 | 0.0285 | 0.0183 | -0.0107 | -0.0225 | -0.0339 | -0.0410 | -0.0461 | -0.0497 | -0.0524 | -0.0544 | -0.0560 | -0.0573 |
| **2.45** | 0.1082 | 0.1248 | 0.1156 | 0.0972 | 0.0763 | 0.0562 | 0.0382 | 0.0230 | 0.0104 | 0.0001 | -0.0279 | -0.0389 | -0.0493 | -0.0559 | -0.0607 | -0.0642 | -0.0668 | -0.0688 | -0.0703 | -0.0715 |
| **2.50** | 0.1063 | 0.1193 | 0.1064 | 0.0850 | 0.0619 | 0.0403 | 0.0215 | 0.0058 | -0.0069 | -0.0170 | -0.0442 | -0.0545 | -0.0641 | -0.0702 | -0.0747 | -0.0780 | -0.0805 | -0.0825 | -0.0840 | -0.0852 |
| **2.55** | 0.1044 | 0.1138 | 0.0973 | 0.0730 | 0.0478 | 0.0249 | 0.0054 | -0.0105 | -0.0232 | -0.0333 | -0.0597 | -0.0694 | -0.0783 | -0.0839 | -0.0881 | -0.0913 | -0.0937 | -0.0956 | -0.0971 | -0.0982 |
| **2.60** | 0.1026 | 0.1083 | 0.0883 | 0.0612 | 0.0341 | 0.0101 | -0.0099 | -0.0261 | -0.0388 | -0.0487 | -0.0744 | -0.0836 | -0.0918 | -0.0970 | -0.1010 | -0.1040 | -0.1063 | -0.1082 | -0.1096 | -0.1108 |
| **2.65** | 0.1007 | 0.1028 | 0.0793 | 0.0496 | 0.0208 | -0.0042 | -0.0246 | -0.0409 | -0.0535 | -0.0633 | -0.0883 | -0.0972 | -0.1049 | -0.1096 | -0.1133 | -0.1162 | -0.1185 | -0.1202 | -0.1216 | -0.1228 |
| **2.70** | 0.0988 | 0.0974 | 0.0705 | 0.0383 | 0.0079 | -0.0179 | -0.0387 | -0.0550 | -0.0675 | -0.0772 | -0.1015 | -0.1102 | -0.1174 | -0.1217 | -0.1252 | -0.1280 | -0.1301 | -0.1318 | -0.1332 | -0.1343 |
| **2.75** | 0.0969 | 0.0920 | 0.0618 | 0.0271 | -0.0047 | -0.0312 | -0.0522 | -0.0684 | -0.0808 | -0.0903 | -0.1142 | -0.1226 | -0.1294 | -0.1334 | -0.1366 | -0.1392 | -0.1413 | -0.1430 | -0.1443 | -0.1454 |
| **2.80** | 0.0951 | 0.0866 | 0.0532 | 0.0163 | -0.0168 | -0.0439 | -0.0650 | -0.0812 | -0.0935 | -0.1028 | -0.1262 | -0.1345 | -0.1410 | -0.1447 | -0.1477 | -0.1501 | -0.1521 | -0.1537 | -0.1550 | -0.1561 |
| **2.85** | 0.0932 | 0.0812 | 0.0447 | 0.0056 | -0.0286 | -0.0561 | -0.0773 | -0.0934 | -0.1055 | -0.1147 | -0.1377 | -0.1459 | -0.1521 | -0.1555 | -0.1583 | -0.1606 | -0.1625 | -0.1641 | -0.1653 | -0.1664 |
| **2.90** | 0.0913 | 0.0759 | 0.0363 | -0.0048 | -0.0400 | -0.0679 | -0.0891 | -0.1050 | -0.1169 | -0.1260 | -0.1487 | -0.1568 | -0.1628 | -0.1660 | -0.1686 | -0.1707 | -0.1725 | -0.1740 | -0.1753 | -0.1763 |
| **2.95** | 0.0895 | 0.0705 | 0.0280 | -0.0149 | -0.0510 | -0.0792 | -0.1003 | -0.1161 | -0.1278 | -0.1367 | -0.1592 | -0.1673 | -0.1732 | -0.1761 | -0.1785 | -0.1805 | -0.1822 | -0.1837 | -0.1849 | -0.1858 |
| **3.00** | 0.0876 | 0.0652 | 0.0198 | -0.0248 | -0.0617 | -0.0900 | -0.1111 | -0.1266 | -0.1382 | -0.1470 | -0.1692 | -0.1773 | -0.1831 | -0.1859 | -0.1880 | -0.1899 | -0.1916 | -0.1930 | -0.1941 | -0.1951 |
| **3.05** | 0.0857 | 0.0600 | 0.0117 | -0.0345 | -0.0720 | -0.1004 | -0.1214 | -0.1367 | -0.1482 | -0.1568 | -0.1788 | -0.1870 | -0.1927 | -0.1953 | -0.1973 | -0.1991 | -0.2006 | -0.2019 | -0.2030 | -0.2040 |
| **3.10** | 0.0838 | 0.0547 | 0.0038 | -0.0439 | -0.0820 | -0.1104 | -0.1312 | -0.1464 | -0.1577 | -0.1662 | -0.1881 | -0.1962 | -0.2020 | -0.2044 | -0.2063 | -0.2079 | -0.2094 | -0.2106 | -0.2117 | -0.2126 |
| **3.15** | 0.0820 | 0.0495 | -0.0040 | -0.0531 | -0.0916 | -0.1201 | -0.1406 | -0.1556 | -0.1668 | -0.1752 | -0.1969 | -0.2051 | -0.2109 | -0.2133 | -0.2149 | -0.2165 | -0.2178 | -0.2190 | -0.2201 | -0.2209 |
| **3.20** | 0.0801 | 0.0444 | -0.0117 | -0.0621 | -0.1010 | -0.1293 | -0.1497 | -0.1645 | -0.1755 | -0.1838 | -0.2054 | -0.2137 | -0.2196 | -0.2218 | -0.2234 | -0.2248 | -0.2260 | -0.2272 | -0.2282 | -0.2290 |
| **3.25** | 0.0783 | 0.0392 | -0.0193 | -0.0708 | -0.1100 | -0.1382 | -0.1584 | -0.1730 | -0.1838 | -0.1920 | -0.2136 | -0.2220 | -0.2279 | -0.2301 | -0.2315 | -0.2328 | -0.2340 | -0.2351 | -0.2360 | -0.2368 |
| **3.30** | 0.0764 | 0.0341 | -0.0268 | -0.0793 | -0.1187 | -0.1468 | -0.1667 | -0.1812 | -0.1919 | -0.2000 | -0.2215 | -0.2300 | -0.2360 | -0.2381 | -0.2394 | -0.2406 | -0.2417 | -0.2427 | -0.2436 | -0.2444 |

| | | | | | | | | | | | | | | | | | | | | |
|---|---|---|---|---|---|---|---|---|---|---|---|---|---|---|---|---|---|---|---|---|
| **3.35** | 0.0745 | 0.0290 | -0.0341 | -0.0876 | -0.1271 | -0.1550 | -0.1748 | -0.1890 | -0.1996 | -0.2076 | -0.2291 | -0.2376 | -0.2437 | -0.2458 | -0.2471 | -0.2482 | -0.2492 | -0.2502 | -0.2510 | -0.2518 |
| **3.40** | 0.0727 | 0.0240 | -0.0413 | -0.0957 | -0.1353 | -0.1630 | -0.1825 | -0.1966 | -0.2070 | -0.2150 | -0.2364 | -0.2451 | -0.2513 | -0.2533 | -0.2545 | -0.2555 | -0.2565 | -0.2574 | -0.2582 | -0.2589 |
| **3.45** | 0.0708 | 0.0190 | -0.0484 | -0.1035 | -0.1432 | -0.1707 | -0.1900 | -0.2039 | -0.2142 | -0.2221 | -0.2435 | -0.2522 | -0.2586 | -0.2606 | -0.2618 | -0.2627 | -0.2636 | -0.2644 | -0.2652 | -0.2658 |
| **3.50** | 0.0690 | 0.0140 | -0.0554 | -0.1112 | -0.1508 | -0.1781 | -0.1972 | -0.2109 | -0.2211 | -0.2290 | -0.2503 | -0.2591 | -0.2656 | -0.2677 | -0.2688 | -0.2696 | -0.2704 | -0.2712 | -0.2719 | -0.2726 |
| **3.55** | 0.0671 | 0.0090 | -0.0622 | -0.1186 | -0.1582 | -0.1853 | -0.2041 | -0.2177 | -0.2278 | -0.2356 | -0.2569 | -0.2658 | -0.2724 | -0.2746 | -0.2756 | -0.2764 | -0.2771 | -0.2778 | -0.2785 | -0.2791 |
| **3.60** | 0.0652 | 0.0041 | -0.0690 | -0.1259 | -0.1654 | -0.1922 | -0.2108 | -0.2242 | -0.2342 | -0.2420 | -0.2633 | -0.2723 | -0.2790 | -0.2812 | -0.2822 | -0.2830 | -0.2836 | -0.2843 | -0.2849 | -0.2855 |
| **3.65** | 0.0634 | -0.0007 | -0.0756 | -0.1330 | -0.1723 | -0.1989 | -0.2173 | -0.2306 | -0.2405 | -0.2482 | -0.2695 | -0.2785 | -0.2854 | -0.2877 | -0.2887 | -0.2894 | -0.2900 | -0.2906 | -0.2912 | -0.2917 |
| **3.70** | 0.0615 | -0.0056 | -0.0821 | -0.1399 | -0.1790 | -0.2053 | -0.2236 | -0.2367 | -0.2466 | -0.2542 | -0.2755 | -0.2846 | -0.2916 | -0.2939 | -0.2949 | -0.2956 | -0.2962 | -0.2967 | -0.2973 | -0.2978 |
| **3.75** | 0.0597 | -0.0104 | -0.0885 | -0.1466 | -0.1856 | -0.2116 | -0.2296 | -0.2426 | -0.2524 | -0.2600 | -0.2813 | -0.2904 | -0.2976 | -0.3000 | -0.3010 | -0.3016 | -0.3022 | -0.3027 | -0.3032 | -0.3037 |
| **3.80** | 0.0578 | -0.0151 | -0.0948 | -0.1531 | -0.1919 | -0.2177 | -0.2355 | -0.2484 | -0.2581 | -0.2657 | -0.2869 | -0.2961 | -0.3035 | -0.3059 | -0.3069 | -0.3075 | -0.3080 | -0.3085 | -0.3090 | -0.3094 |
| **3.85** | 0.0560 | -0.0199 | -0.1010 | -0.1595 | -0.1981 | -0.2236 | -0.2413 | -0.2540 | -0.2637 | -0.2712 | -0.2924 | -0.3017 | -0.3091 | -0.3117 | -0.3127 | -0.3133 | -0.3138 | -0.3142 | -0.3146 | -0.3150 |
| **3.90** | 0.0542 | -0.0245 | -0.1070 | -0.1657 | -0.2041 | -0.2293 | -0.2468 | -0.2595 | -0.2691 | -0.2765 | -0.2977 | -0.3070 | -0.3146 | -0.3172 | -0.3183 | -0.3189 | -0.3193 | -0.3197 | -0.3201 | -0.3205 |
| **3.95** | 0.0523 | -0.0292 | -0.1130 | -0.1718 | -0.2099 | -0.2349 | -0.2522 | -0.2648 | -0.2743 | -0.2817 | -0.3028 | -0.3123 | -0.3200 | -0.3227 | -0.3238 | -0.3243 | -0.3248 | -0.3251 | -0.3255 | -0.3259 |
| **4.00** | 0.0505 | -0.0338 | -0.1188 | -0.1777 | -0.2155 | -0.2403 | -0.2575 | -0.2699 | -0.2794 | -0.2868 | -0.3079 | -0.3173 | -0.3252 | -0.3279 | -0.3291 | -0.3297 | -0.3301 | -0.3304 | -0.3307 | -0.3311 |
| **4.05** | 0.0486 | -0.0384 | -0.1245 | -0.1835 | -0.2210 | -0.2456 | -0.2626 | -0.2750 | -0.2843 | -0.2917 | -0.3127 | -0.3223 | -0.3302 | -0.3331 | -0.3343 | -0.3349 | -0.3352 | -0.3355 | -0.3359 | -0.3362 |
| **4.10** | 0.0468 | -0.0429 | -0.1302 | -0.1891 | -0.2264 | -0.2508 | -0.2676 | -0.2799 | -0.2892 | -0.2965 | -0.3175 | -0.3271 | -0.3351 | -0.3381 | -0.3393 | -0.3399 | -0.3403 | -0.3406 | -0.3409 | -0.3411 |
| **4.15** | 0.0450 | -0.0474 | -0.1357 | -0.1946 | -0.2316 | -0.2558 | -0.2724 | -0.2846 | -0.2939 | -0.3012 | -0.3222 | -0.3317 | -0.3399 | -0.3429 | -0.3442 | -0.3448 | -0.3452 | -0.3455 | -0.3458 | -0.3460 |
| **4.20** | 0.0431 | -0.0519 | -0.1411 | -0.2000 | -0.2367 | -0.2606 | -0.2772 | -0.2893 | -0.2985 | -0.3058 | -0.3267 | -0.3363 | -0.3446 | -0.3477 | -0.3490 | -0.3497 | -0.3500 | -0.3503 | -0.3505 | -0.3508 |
| **4.25** | 0.0413 | -0.0563 | -0.1465 | -0.2052 | -0.2417 | -0.2654 | -0.2818 | -0.2938 | -0.3030 | -0.3102 | -0.3311 | -0.3407 | -0.3491 | -0.3523 | -0.3537 | -0.3543 | -0.3547 | -0.3550 | -0.3552 | -0.3554 |
| **4.30** | 0.0395 | -0.0607 | -0.1517 | -0.2104 | -0.2465 | -0.2700 | -0.2863 | -0.2983 | -0.3074 | -0.3146 | -0.3354 | -0.3451 | -0.3535 | -0.3568 | -0.3582 | -0.3589 | -0.3593 | -0.3596 | -0.3598 | -0.3600 |
| **4.35** | 0.0376 | -0.0650 | -0.1569 | -0.2154 | -0.2513 | -0.2746 | -0.2907 | -0.3026 | -0.3117 | -0.3189 | -0.3396 | -0.3493 | -0.3578 | -0.3612 | -0.3627 | -0.3634 | -0.3638 | -0.3640 | -0.3642 | -0.3644 |
| **4.40** | 0.0358 | -0.0693 | -0.1619 | -0.2203 | -0.2559 | -0.2790 | -0.2951 | -0.3069 | -0.3159 | -0.3230 | -0.3437 | -0.3534 | -0.3621 | -0.3655 | -0.3670 | -0.3678 | -0.3682 | -0.3684 | -0.3686 | -0.3688 |
| **4.45** | 0.0340 | -0.0736 | -0.1669 | -0.2250 | -0.2604 | -0.2834 | -0.2993 | -0.3110 | -0.3200 | -0.3271 | -0.3478 | -0.3575 | -0.3662 | -0.3697 | -0.3712 | -0.3720 | -0.3724 | -0.3727 | -0.3729 | -0.3731 |
| **4.50** | 0.0322 | -0.0778 | -0.1718 | -0.2297 | -0.2648 | -0.2876 | -0.3034 | -0.3151 | -0.3240 | -0.3311 | -0.3517 | -0.3614 | -0.3702 | -0.3737 | -0.3754 | -0.3762 | -0.3766 | -0.3769 | -0.3771 | -0.3772 |

## (A.2) Force-extension relation of a half-clamped semiflexible polymer with different persistence lengths $l_P$ and forces F

| | persistence length $l_P/L$ | | | | | | | | | | | | | | | | | | | |
|---|---|---|---|---|---|---|---|---|---|---|---|---|---|---|---|---|---|---|---|---|
| $\lvert F\rvert/F_c$ | **0.1** | **0.2** | **0.3** | **0.4** | **0.5** | **0.6** | **0.8** | **1.0** | **1.2** | **1.4** | **1.6** | **2.0** | **3.0** | **4.0** | **6.0** | **8.0** | **10.0** | **12.0** | **16.0** | **20.0** |
| **0.00** | 0.1000 | 0.1986 | 0.2892 | 0.3671 | 0.4323 | 0.4866 | 0.5707 | 0.6321 | 0.6784 | 0.7146 | 0.7436 | 0.7869 | 0.8504 | 0.8848 | 0.9211 | 0.9400 | 0.9516 | 0.9595 | 0.9694 | 0.9754 |
| **0.05** | 0.0994 | 0.1970 | 0.2864 | 0.3633 | 0.4277 | 0.4814 | 0.5649 | 0.6260 | 0.6723 | 0.7086 | 0.7377 | 0.7815 | 0.8459 | 0.8810 | 0.9183 | 0.9378 | 0.9498 | 0.9579 | 0.9682 | 0.9744 |
| **0.10** | 0.0989 | 0.1954 | 0.2836 | 0.3595 | 0.4230 | 0.4762 | 0.5590 | 0.6198 | 0.6661 | 0.7024 | 0.7316 | 0.7757 | 0.8411 | 0.8769 | 0.9152 | 0.9353 | 0.9477 | 0.9561 | 0.9668 | 0.9733 |
| **0.15** | 0.0984 | 0.1937 | 0.2808 | 0.3556 | 0.4184 | 0.4709 | 0.5530 | 0.6134 | 0.6596 | 0.6959 | 0.7253 | 0.7697 | 0.8360 | 0.8726 | 0.9119 | 0.9326 | 0.9455 | 0.9542 | 0.9653 | 0.9721 |
| **0.20** | 0.0979 | 0.1921 | 0.2780 | 0.3517 | 0.4137 | 0.4656 | 0.5468 | 0.6069 | 0.6529 | 0.6893 | 0.7187 | 0.7634 | 0.8306 | 0.8679 | 0.9083 | 0.9297 | 0.9430 | 0.9521 | 0.9637 | 0.9707 |
| **0.25** | 0.0974 | 0.1905 | 0.2752 | 0.3478 | 0.4089 | 0.4602 | 0.5406 | 0.6002 | 0.6460 | 0.6823 | 0.7118 | 0.7568 | 0.8248 | 0.8629 | 0.9044 | 0.9265 | 0.9403 | 0.9498 | 0.9618 | 0.9692 |

| | | | | | | | | | | | | | | | | | | | | |
|---|---|---|---|---|---|---|---|---|---|---|---|---|---|---|---|---|---|---|---|---|
| **0.30** | 0.0969 | 0.1889 | 0.2723 | 0.3439 | 0.4041 | 0.4547 | 0.5342 | 0.5933 | 0.6389 | 0.6752 | 0.7047 | 0.7499 | 0.8186 | 0.8575 | 0.9001 | 0.9230 | 0.9373 | 0.9472 | 0.9598 | 0.9675 |
| **0.35** | 0.0964 | 0.1873 | 0.2695 | 0.3400 | 0.3993 | 0.4492 | 0.5277 | 0.5863 | 0.6316 | 0.6678 | 0.6973 | 0.7426 | 0.8121 | 0.8517 | 0.8954 | 0.9191 | 0.9340 | 0.9443 | 0.9575 | 0.9656 |
| **0.40** | 0.0959 | 0.1856 | 0.2666 | 0.3361 | 0.3945 | 0.4436 | 0.5211 | 0.5791 | 0.6241 | 0.6601 | 0.6896 | 0.7350 | 0.8051 | 0.8454 | 0.8902 | 0.9148 | 0.9303 | 0.9410 | 0.9549 | 0.9634 |
| **0.45** | 0.0954 | 0.1840 | 0.2638 | 0.3321 | 0.3896 | 0.4380 | 0.5144 | 0.5718 | 0.6164 | 0.6522 | 0.6816 | 0.7270 | 0.7977 | 0.8386 | 0.8846 | 0.9100 | 0.9261 | 0.9373 | 0.9519 | 0.9609 |
| **0.50** | 0.0949 | 0.1824 | 0.2609 | 0.3281 | 0.3846 | 0.4323 | 0.5076 | 0.5643 | 0.6085 | 0.6440 | 0.6732 | 0.7187 | 0.7897 | 0.8313 | 0.8784 | 0.9046 | 0.9214 | 0.9332 | 0.9485 | 0.9581 |
| **0.55** | 0.0944 | 0.1808 | 0.2581 | 0.3241 | 0.3797 | 0.4265 | 0.5007 | 0.5566 | 0.6003 | 0.6355 | 0.6646 | 0.7099 | 0.7812 | 0.8233 | 0.8715 | 0.8986 | 0.9161 | 0.9284 | 0.9446 | 0.9547 |
| **0.60** | 0.0938 | 0.1791 | 0.2552 | 0.3201 | 0.3747 | 0.4207 | 0.4937 | 0.5488 | 0.5919 | 0.6268 | 0.6556 | 0.7007 | 0.7722 | 0.8147 | 0.8639 | 0.8919 | 0.9101 | 0.9230 | 0.9400 | 0.9511 |
| **0.65** | 0.0933 | 0.1775 | 0.2523 | 0.3160 | 0.3696 | 0.4149 | 0.4865 | 0.5408 | 0.5833 | 0.6178 | 0.6463 | 0.6911 | 0.7625 | 0.8054 | 0.8555 | 0.8843 | 0.9033 | 0.9167 | 0.9347 | 0.9462 |
| **0.70** | 0.0928 | 0.1759 | 0.2494 | 0.3120 | 0.3646 | 0.4089 | 0.4793 | 0.5326 | 0.5745 | 0.6085 | 0.6367 | 0.6810 | 0.7522 | 0.7953 | 0.8462 | 0.8758 | 0.8954 | 0.9095 | 0.9284 | 0.9406 |
| **0.75** | 0.0923 | 0.1742 | 0.2465 | 0.3079 | 0.3595 | 0.4030 | 0.4719 | 0.5242 | 0.5654 | 0.5989 | 0.6267 | 0.6705 | 0.7412 | 0.7844 | 0.8358 | 0.8661 | 0.8864 | 0.9010 | 0.9214 | 0.9339 |
| **0.80** | 0.0918 | 0.1726 | 0.2436 | 0.3038 | 0.3543 | 0.3969 | 0.4645 | 0.5157 | 0.5561 | 0.5890 | 0.6163 | 0.6595 | 0.7295 | 0.7726 | 0.8243 | 0.8551 | 0.8759 | 0.8911 | 0.9119 | 0.9257 |
| **0.85** | 0.0913 | 0.1710 | 0.2407 | 0.2997 | 0.3492 | 0.3908 | 0.4569 | 0.5070 | 0.5466 | 0.5788 | 0.6056 | 0.6480 | 0.7171 | 0.7598 | 0.8115 | 0.8426 | 0.8638 | 0.8794 | 0.9013 | 0.9156 |
| **0.90** | 0.0908 | 0.1694 | 0.2378 | 0.2956 | 0.3440 | 0.3847 | 0.4492 | 0.4982 | 0.5368 | 0.5683 | 0.5945 | 0.6360 | 0.7038 | 0.7459 | 0.7973 | 0.8284 | 0.8498 | 0.8657 | 0.8879 | 0.9030 |
| **0.95** | 0.0903 | 0.1677 | 0.2349 | 0.2915 | 0.3388 | 0.3785 | 0.4415 | 0.4892 | 0.5268 | 0.5575 | 0.5830 | 0.6235 | 0.6898 | 0.7310 | 0.7815 | 0.8123 | 0.8336 | 0.8494 | 0.8718 | 0.8872 |
| **1.00** | 0.0898 | 0.1661 | 0.2320 | 0.2873 | 0.3335 | 0.3723 | 0.4336 | 0.4800 | 0.5166 | 0.5464 | 0.5712 | 0.6105 | 0.6748 | 0.7149 | 0.7639 | 0.7940 | 0.8148 | 0.8303 | 0.8523 | 0.8674 |
| **1.05** | 0.0893 | 0.1644 | 0.2291 | 0.2832 | 0.3282 | 0.3660 | 0.4256 | 0.4707 | 0.5062 | 0.5350 | 0.5590 | 0.5970 | 0.6590 | 0.6976 | 0.7446 | 0.7733 | 0.7930 | 0.8084 | 0.8285 | 0.8426 |
| **1.10** | 0.0887 | 0.1628 | 0.2261 | 0.2790 | 0.3229 | 0.3597 | 0.4176 | 0.4612 | 0.4955 | 0.5234 | 0.5465 | 0.5830 | 0.6424 | 0.6790 | 0.7233 | 0.7500 | 0.7681 | 0.7814 | 0.7998 | 0.8119 |
| **1.15** | 0.0882 | 0.1612 | 0.2232 | 0.2748 | 0.3176 | 0.3533 | 0.4094 | 0.4516 | 0.4847 | 0.5114 | 0.5336 | 0.5685 | 0.6248 | 0.6591 | 0.7000 | 0.7239 | 0.7397 | 0.7510 | 0.7657 | 0.7746 |
| **1.20** | 0.0877 | 0.1595 | 0.2203 | 0.2706 | 0.3122 | 0.3469 | 0.4012 | 0.4418 | 0.4736 | 0.4992 | 0.5203 | 0.5535 | 0.6063 | 0.6380 | 0.6746 | 0.6950 | 0.7078 | 0.7163 | 0.7260 | 0.7305 |
| **1.25** | 0.0872 | 0.1579 | 0.2173 | 0.2664 | 0.3068 | 0.3404 | 0.3928 | 0.4319 | 0.4623 | 0.4866 | 0.5067 | 0.5379 | 0.5869 | 0.6155 | 0.6471 | 0.6633 | 0.6724 | 0.6775 | 0.6812 | 0.6805 |
| **1.30** | 0.0867 | 0.1562 | 0.2144 | 0.2622 | 0.3014 | 0.3339 | 0.3844 | 0.4218 | 0.4508 | 0.4739 | 0.4928 | 0.5219 | 0.5667 | 0.5918 | 0.6177 | 0.6290 | 0.6338 | 0.6350 | 0.6322 | 0.6264 |
| **1.35** | 0.0862 | 0.1546 | 0.2114 | 0.2579 | 0.2960 | 0.3274 | 0.3759 | 0.4116 | 0.4391 | 0.4608 | 0.4785 | 0.5054 | 0.5456 | 0.5669 | 0.5864 | 0.5924 | 0.5925 | 0.5898 | 0.5807 | 0.5705 |
| **1.40** | 0.0857 | 0.1530 | 0.2085 | 0.2537 | 0.2905 | 0.3208 | 0.3673 | 0.4013 | 0.4272 | 0.4475 | 0.4639 | 0.4885 | 0.5238 | 0.5410 | 0.5535 | 0.5538 | 0.5493 | 0.5428 | 0.5285 | 0.5154 |
| **1.45** | 0.0852 | 0.1513 | 0.2055 | 0.2494 | 0.2850 | 0.3142 | 0.3587 | 0.3909 | 0.4151 | 0.4340 | 0.4490 | 0.4712 | 0.5012 | 0.5140 | 0.5193 | 0.5140 | 0.5051 | 0.4954 | 0.4773 | 0.4629 |
| **1.50** | 0.0847 | 0.1497 | 0.2025 | 0.2452 | 0.2795 | 0.3075 | 0.3499 | 0.3803 | 0.4029 | 0.4203 | 0.4339 | 0.4535 | 0.4780 | 0.4862 | 0.4841 | 0.4738 | 0.4608 | 0.4486 | 0.4284 | 0.4141 |
| **1.55** | 0.0842 | 0.1480 | 0.1996 | 0.2409 | 0.2740 | 0.3008 | 0.3411 | 0.3696 | 0.3905 | 0.4063 | 0.4185 | 0.4354 | 0.4542 | 0.4577 | 0.4484 | 0.4328 | 0.4172 | 0.4035 | 0.3827 | 0.3692 |
| **1.60** | 0.0836 | 0.1464 | 0.1966 | 0.2366 | 0.2685 | 0.2941 | 0.3323 | 0.3588 | 0.3780 | 0.3922 | 0.4028 | 0.4169 | 0.4300 | 0.4287 | 0.4124 | 0.3928 | 0.3751 | 0.3607 | 0.3405 | 0.3282 |
| **1.65** | 0.0831 | 0.1447 | 0.1936 | 0.2323 | 0.2629 | 0.2873 | 0.3233 | 0.3480 | 0.3653 | 0.3779 | 0.3870 | 0.3983 | 0.4053 | 0.3994 | 0.3768 | 0.3538 | 0.3350 | 0.3205 | 0.3015 | 0.2906 |
| **1.70** | 0.0826 | 0.1431 | 0.1907 | 0.2280 | 0.2573 | 0.2806 | 0.3144 | 0.3370 | 0.3525 | 0.3634 | 0.3709 | 0.3793 | 0.3804 | 0.3699 | 0.3417 | 0.3165 | 0.2972 | 0.2832 | 0.2657 | 0.2559 |
| **1.75** | 0.0821 | 0.1415 | 0.1877 | 0.2237 | 0.2517 | 0.2738 | 0.3053 | 0.3259 | 0.3396 | 0.3488 | 0.3547 | 0.3602 | 0.3554 | 0.3406 | 0.3076 | 0.2809 | 0.2618 | 0.2486 | 0.2327 | 0.2239 |
| **1.80** | 0.0816 | 0.1398 | 0.1847 | 0.2194 | 0.2461 | 0.2669 | 0.2962 | 0.3148 | 0.3266 | 0.3340 | 0.3383 | 0.3409 | 0.3303 | 0.3115 | 0.2746 | 0.2473 | 0.2288 | 0.2165 | 0.2020 | 0.1941 |
| **1.85** | 0.0811 | 0.1382 | 0.1817 | 0.2150 | 0.2405 | 0.2601 | 0.2871 | 0.3036 | 0.3136 | 0.3192 | 0.3219 | 0.3215 | 0.3053 | 0.2829 | 0.2430 | 0.2157 | 0.1981 | 0.1868 | 0.1736 | 0.1663 |
| **1.90** | 0.0806 | 0.1365 | 0.1787 | 0.2107 | 0.2349 | 0.2532 | 0.2780 | 0.2924 | 0.3004 | 0.3043 | 0.3053 | 0.3021 | 0.2805 | 0.2549 | 0.2129 | 0.1860 | 0.1696 | 0.1591 | 0.1470 | 0.1402 |
| **1.95** | 0.0801 | 0.1349 | 0.1757 | 0.2063 | 0.2292 | 0.2463 | 0.2688 | 0.2811 | 0.2872 | 0.2893 | 0.2887 | 0.2827 | 0.2559 | 0.2276 | 0.1843 | 0.1583 | 0.1429 | 0.1333 | 0.1221 | 0.1158 |
| **2.00** | 0.0796 | 0.1332 | 0.1727 | 0.2020 | 0.2236 | 0.2394 | 0.2595 | 0.2697 | 0.2739 | 0.2743 | 0.2721 | 0.2633 | 0.2318 | 0.2011 | 0.1573 | 0.1324 | 0.1180 | 0.1091 | 0.0987 | 0.0928 |
| **2.05** | 0.0791 | 0.1316 | 0.1698 | 0.1977 | 0.2179 | 0.2325 | 0.2503 | 0.2584 | 0.2607 | 0.2593 | 0.2555 | 0.2440 | 0.2081 | 0.1756 | 0.1317 | 0.1081 | 0.0947 | 0.0864 | 0.0766 | 0.0710 |
| **2.10** | 0.0785 | 0.1299 | 0.1668 | 0.1933 | 0.2122 | 0.2256 | 0.2410 | 0.2470 | 0.2474 | 0.2442 | 0.2390 | 0.2248 | 0.1850 | 0.1511 | 0.1077 | 0.0853 | 0.0728 | 0.0650 | 0.0558 | 0.0505 |

| | | | | | | | | | | | | | | | | | | | | |
|---|---|---|---|---|---|---|---|---|---|---|---|---|---|---|---|---|---|---|---|---|
| **2.15** | 0.0780 | 0.1283 | 0.1638 | 0.1889 | 0.2065 | 0.2186 | 0.2317 | 0.2356 | 0.2341 | 0.2293 | 0.2225 | 0.2059 | 0.1625 | 0.1275 | 0.0851 | 0.0639 | 0.0522 | 0.0448 | 0.0361 | 0.0311 |
| **2.20** | 0.0775 | 0.1266 | 0.1608 | 0.1846 | 0.2008 | 0.2117 | 0.2224 | 0.2242 | 0.2208 | 0.2143 | 0.2061 | 0.1871 | 0.1406 | 0.1051 | 0.0637 | 0.0437 | 0.0327 | 0.0257 | 0.0174 | 0.0126 |
| **2.25** | 0.0770 | 0.1250 | 0.1578 | 0.1802 | 0.1952 | 0.2047 | 0.2131 | 0.2128 | 0.2075 | 0.1994 | 0.1898 | 0.1686 | 0.1194 | 0.0836 | 0.0436 | 0.0247 | 0.0142 | 0.0076 | -0.0003 | -0.0049 |
| **2.30** | 0.0765 | 0.1233 | 0.1548 | 0.1758 | 0.1895 | 0.1977 | 0.2038 | 0.2014 | 0.1943 | 0.1847 | 0.1737 | 0.1504 | 0.0990 | 0.0631 | 0.0246 | 0.0067 | -0.0032 | -0.0095 | -0.0172 | -0.0216 |
| **2.35** | 0.0760 | 0.1217 | 0.1518 | 0.1715 | 0.1838 | 0.1908 | 0.1945 | 0.1901 | 0.1812 | 0.1700 | 0.1577 | 0.1326 | 0.0793 | 0.0437 | 0.0066 | -0.0104 | -0.0198 | -0.0259 | -0.0332 | -0.0375 |
| **2.40** | 0.0755 | 0.1200 | 0.1488 | 0.1671 | 0.1781 | 0.1838 | 0.1852 | 0.1787 | 0.1681 | 0.1554 | 0.1419 | 0.1151 | 0.0603 | 0.0252 | -0.0105 | -0.0266 | -0.0356 | -0.0414 | -0.0485 | -0.0526 |
| **2.45** | 0.0750 | 0.1184 | 0.1458 | 0.1627 | 0.1724 | 0.1768 | 0.1759 | 0.1675 | 0.1551 | 0.1410 | 0.1264 | 0.0980 | 0.0421 | 0.0075 | -0.0266 | -0.0420 | -0.0507 | -0.0563 | -0.0631 | -0.0671 |
| **2.50** | 0.0745 | 0.1167 | 0.1428 | 0.1584 | 0.1667 | 0.1699 | 0.1667 | 0.1562 | 0.1422 | 0.1268 | 0.1111 | 0.0812 | 0.0246 | -0.0092 | -0.0420 | -0.0567 | -0.0651 | -0.0705 | -0.0771 | -0.0809 |
| **2.55** | 0.0740 | 0.1151 | 0.1398 | 0.1540 | 0.1610 | 0.1629 | 0.1575 | 0.1451 | 0.1295 | 0.1127 | 0.0960 | 0.0649 | 0.0078 | -0.0252 | -0.0566 | -0.0708 | -0.0788 | -0.0840 | -0.0904 | -0.0942 |
| **2.60** | 0.0734 | 0.1134 | 0.1368 | 0.1496 | 0.1553 | 0.1560 | 0.1483 | 0.1339 | 0.1168 | 0.0989 | 0.0812 | 0.0491 | -0.0083 | -0.0404 | -0.0705 | -0.0842 | -0.0919 | -0.0970 | -0.1032 | -0.1069 |
| **2.65** | 0.0729 | 0.1118 | 0.1338 | 0.1452 | 0.1496 | 0.1490 | 0.1391 | 0.1229 | 0.1043 | 0.0852 | 0.0667 | 0.0336 | -0.0237 | -0.0549 | -0.0838 | -0.0970 | -0.1045 | -0.1094 | -0.1155 | -0.1190 |
| **2.70** | 0.0724 | 0.1101 | 0.1308 | 0.1409 | 0.1439 | 0.1421 | 0.1300 | 0.1120 | 0.0919 | 0.0717 | 0.0525 | 0.0186 | -0.0384 | -0.0687 | -0.0966 | -0.1093 | -0.1166 | -0.1214 | -0.1273 | -0.1307 |
| **2.75** | 0.0719 | 0.1085 | 0.1278 | 0.1365 | 0.1382 | 0.1352 | 0.1209 | 0.1011 | 0.0797 | 0.0585 | 0.0386 | 0.0041 | -0.0525 | -0.0819 | -0.1088 | -0.1211 | -0.1282 | -0.1328 | -0.1386 | -0.1420 |
| **2.80** | 0.0714 | 0.1068 | 0.1248 | 0.1321 | 0.1325 | 0.1283 | 0.1118 | 0.0903 | 0.0676 | 0.0455 | 0.0250 | -0.0101 | -0.0660 | -0.0945 | -0.1204 | -0.1324 | -0.1393 | -0.1439 | -0.1494 | -0.1528 |
| **2.85** | 0.0709 | 0.1052 | 0.1218 | 0.1278 | 0.1269 | 0.1214 | 0.1028 | 0.0797 | 0.0557 | 0.0328 | 0.0117 | -0.0237 | -0.0790 | -0.1066 | -0.1317 | -0.1433 | -0.1500 | -0.1544 | -0.1599 | -0.1632 |
| **2.90** | 0.0704 | 0.1035 | 0.1188 | 0.1234 | 0.1212 | 0.1146 | 0.0939 | 0.0691 | 0.0440 | 0.0202 | -0.0013 | -0.0370 | -0.0914 | -0.1181 | -0.1424 | -0.1537 | -0.1603 | -0.1646 | -0.1700 | -0.1732 |
| **2.95** | 0.0699 | 0.1019 | 0.1158 | 0.1191 | 0.1156 | 0.1077 | 0.0850 | 0.0587 | 0.0324 | 0.0080 | -0.0139 | -0.0498 | -0.1033 | -0.1292 | -0.1528 | -0.1638 | -0.1703 | -0.1745 | -0.1797 | -0.1828 |
| **3.00** | 0.0694 | 0.1002 | 0.1128 | 0.1147 | 0.1099 | 0.1009 | 0.0762 | 0.0484 | 0.0211 | -0.0040 | -0.0263 | -0.0622 | -0.1147 | -0.1399 | -0.1628 | -0.1735 | -0.1798 | -0.1840 | -0.1891 | -0.1921 |
| **3.05** | 0.0688 | 0.0986 | 0.1098 | 0.1104 | 0.1043 | 0.0941 | 0.0674 | 0.0382 | 0.0099 | -0.0157 | -0.0383 | -0.0741 | -0.1257 | -0.1501 | -0.1724 | -0.1829 | -0.1891 | -0.1931 | -0.1981 | -0.2011 |
| **3.10** | 0.0683 | 0.0969 | 0.1068 | 0.1061 | 0.0987 | 0.0873 | 0.0588 | 0.0281 | -0.0010 | -0.0272 | -0.0499 | -0.0857 | -0.1362 | -0.1599 | -0.1816 | -0.1919 | -0.1980 | -0.2020 | -0.2069 | -0.2098 |
| **3.15** | 0.0678 | 0.0953 | 0.1038 | 0.1017 | 0.0931 | 0.0806 | 0.0501 | 0.0182 | -0.0118 | -0.0384 | -0.0613 | -0.0969 | -0.1464 | -0.1694 | -0.1906 | -0.2007 | -0.2066 | -0.2105 | -0.2153 | -0.2182 |
| **3.20** | 0.0673 | 0.0936 | 0.1008 | 0.0974 | 0.0875 | 0.0739 | 0.0416 | 0.0084 | -0.0224 | -0.0493 | -0.0723 | -0.1077 | -0.1561 | -0.1785 | -0.1992 | -0.2091 | -0.2149 | -0.2188 | -0.2235 | -0.2263 |
| **3.25** | 0.0668 | 0.0920 | 0.0978 | 0.0931 | 0.0820 | 0.0672 | 0.0331 | -0.0013 | -0.0327 | -0.0600 | -0.0831 | -0.1181 | -0.1655 | -0.1874 | -0.2076 | -0.2173 | -0.2230 | -0.2268 | -0.2314 | -0.2342 |
| **3.30** | 0.0663 | 0.0903 | 0.0949 | 0.0888 | 0.0764 | 0.0606 | 0.0248 | -0.0108 | -0.0429 | -0.0704 | -0.0935 | -0.1282 | -0.1746 | -0.1959 | -0.2157 | -0.2252 | -0.2308 | -0.2345 | -0.2391 | -0.2418 |
| **3.35** | 0.0658 | 0.0887 | 0.0919 | 0.0845 | 0.0709 | 0.0540 | 0.0165 | -0.0202 | -0.0528 | -0.0806 | -0.1036 | -0.1380 | -0.1833 | -0.2041 | -0.2235 | -0.2328 | -0.2384 | -0.2420 | -0.2465 | -0.2492 |
| **3.40** | 0.0653 | 0.0870 | 0.0889 | 0.0802 | 0.0654 | 0.0474 | 0.0083 | -0.0294 | -0.0626 | -0.0905 | -0.1135 | -0.1474 | -0.1918 | -0.2121 | -0.2311 | -0.2403 | -0.2457 | -0.2493 | -0.2537 | -0.2564 |
| **3.45** | 0.0648 | 0.0854 | 0.0859 | 0.0759 | 0.0599 | 0.0409 | 0.0001 | -0.0385 | -0.0721 | -0.1001 | -0.1230 | -0.1565 | -0.1999 | -0.2198 | -0.2384 | -0.2475 | -0.2528 | -0.2563 | -0.2607 | -0.2633 |
| **3.50** | 0.0643 | 0.0837 | 0.0830 | 0.0716 | 0.0545 | 0.0344 | -0.0079 | -0.0474 | -0.0814 | -0.1095 | -0.1323 | -0.1653 | -0.2078 | -0.2272 | -0.2456 | -0.2545 | -0.2597 | -0.2632 | -0.2675 | -0.2701 |
| **3.55** | 0.0637 | 0.0821 | 0.0800 | 0.0674 | 0.0490 | 0.0280 | -0.0158 | -0.0562 | -0.0906 | -0.1187 | -0.1413 | -0.1739 | -0.2154 | -0.2345 | -0.2525 | -0.2612 | -0.2664 | -0.2698 | -0.2741 | -0.2766 |
| **3.60** | 0.0632 | 0.0804 | 0.0770 | 0.0631 | 0.0436 | 0.0215 | -0.0237 | -0.0648 | -0.0995 | -0.1276 | -0.1500 | -0.1821 | -0.2228 | -0.2415 | -0.2592 | -0.2678 | -0.2729 | -0.2763 | -0.2805 | -0.2830 |
| **3.65** | 0.0627 | 0.0788 | 0.0741 | 0.0589 | 0.0382 | 0.0152 | -0.0314 | -0.0733 | -0.1082 | -0.1363 | -0.1585 | -0.1901 | -0.2300 | -0.2483 | -0.2657 | -0.2742 | -0.2793 | -0.2826 | -0.2867 | -0.2892 |
| **3.70** | 0.0622 | 0.0771 | 0.0711 | 0.0546 | 0.0329 | 0.0089 | -0.0391 | -0.0816 | -0.1167 | -0.1447 | -0.1667 | -0.1978 | -0.2369 | -0.2549 | -0.2721 | -0.2805 | -0.2854 | -0.2887 | -0.2928 | -0.2953 |
| **3.75** | 0.0617 | 0.0755 | 0.0682 | 0.0504 | 0.0275 | 0.0026 | -0.0467 | -0.0898 | -0.1250 | -0.1529 | -0.1747 | -0.2053 | -0.2437 | -0.2613 | -0.2783 | -0.2865 | -0.2914 | -0.2947 | -0.2987 | -0.3011 |
| **3.80** | 0.0612 | 0.0738 | 0.0652 | 0.0462 | 0.0222 | -0.0036 | -0.0541 | -0.0978 | -0.1332 | -0.1609 | -0.1825 | -0.2126 | -0.2502 | -0.2676 | -0.2843 | -0.2924 | -0.2972 | -0.3005 | -0.3044 | -0.3068 |
| **3.85** | 0.0607 | 0.0722 | 0.0623 | 0.0420 | 0.0169 | -0.0098 | -0.0615 | -0.1057 | -0.1411 | -0.1687 | -0.1900 | -0.2197 | -0.2566 | -0.2737 | -0.2901 | -0.2981 | -0.3029 | -0.3061 | -0.3100 | -0.3124 |
| **3.90** | 0.0602 | 0.0706 | 0.0593 | 0.0378 | 0.0117 | -0.0160 | -0.0687 | -0.1134 | -0.1489 | -0.1763 | -0.1974 | -0.2265 | -0.2627 | -0.2796 | -0.2958 | -0.3037 | -0.3085 | -0.3116 | -0.3155 | -0.3178 |
| **3.95** | 0.0597 | 0.0689 | 0.0564 | 0.0337 | 0.0064 | -0.0220 | -0.0759 | -0.1210 | -0.1564 | -0.1837 | -0.2045 | -0.2331 | -0.2687 | -0.2853 | -0.3013 | -0.3092 | -0.3139 | -0.3170 | -0.3208 | -0.3231 |

| | | | | | | | | | | | | | | | | | | | | |
|---|---|---|---|---|---|---|---|---|---|---|---|---|---|---|---|---|---|---|---|---|
| **4.00** | 0.0591 | 0.0673 | 0.0534 | 0.0295 | 0.0012 | -0.0281 | -0.0830 | -0.1284 | -0.1638 | -0.1908 | -0.2114 | -0.2396 | -0.2746 | -0.2909 | -0.3067 | -0.3145 | -0.3191 | -0.3222 | -0.3260 | -0.3283 |
| **4.05** | 0.0586 | 0.0656 | 0.0505 | 0.0254 | -0.0039 | -0.0341 | -0.0899 | -0.1357 | -0.1710 | -0.1978 | -0.2181 | -0.2459 | -0.2803 | -0.2964 | -0.3120 | -0.3197 | -0.3243 | -0.3273 | -0.3311 | -0.3333 |
| **4.10** | 0.0581 | 0.0640 | 0.0476 | 0.0212 | -0.0091 | -0.0400 | -0.0968 | -0.1428 | -0.1781 | -0.2046 | -0.2247 | -0.2520 | -0.2858 | -0.3017 | -0.3172 | -0.3248 | -0.3293 | -0.3323 | -0.3360 | -0.3382 |
| **4.15** | 0.0576 | 0.0624 | 0.0447 | 0.0171 | -0.0142 | -0.0459 | -0.1035 | -0.1498 | -0.1850 | -0.2113 | -0.2310 | -0.2579 | -0.2912 | -0.3069 | -0.3222 | -0.3297 | -0.3342 | -0.3371 | -0.3408 | -0.3430 |
| **4.20** | 0.0571 | 0.0607 | 0.0418 | 0.0130 | -0.0193 | -0.0517 | -0.1102 | -0.1566 | -0.1917 | -0.2177 | -0.2372 | -0.2637 | -0.2965 | -0.3120 | -0.3271 | -0.3345 | -0.3389 | -0.3419 | -0.3455 | -0.3477 |
| **4.25** | 0.0566 | 0.0591 | 0.0388 | 0.0089 | -0.0243 | -0.0575 | -0.1167 | -0.1634 | -0.1982 | -0.2240 | -0.2433 | -0.2693 | -0.3017 | -0.3170 | -0.3319 | -0.3392 | -0.3436 | -0.3465 | -0.3501 | -0.3523 |
| **4.30** | 0.0561 | 0.0574 | 0.0359 | 0.0049 | -0.0293 | -0.0632 | -0.1232 | -0.1699 | -0.2046 | -0.2302 | -0.2491 | -0.2748 | -0.3067 | -0.3218 | -0.3366 | -0.3438 | -0.3482 | -0.3510 | -0.3546 | -0.3568 |
| **4.35** | 0.0556 | 0.0558 | 0.0330 | 0.0008 | -0.0343 | -0.0688 | -0.1295 | -0.1764 | -0.2109 | -0.2361 | -0.2549 | -0.2801 | -0.3116 | -0.3265 | -0.3411 | -0.3483 | -0.3526 | -0.3555 | -0.3590 | -0.3612 |
| **4.40** | 0.0551 | 0.0542 | 0.0301 | -0.0032 | -0.0393 | -0.0745 | -0.1358 | -0.1827 | -0.2170 | -0.2420 | -0.2604 | -0.2853 | -0.3164 | -0.3312 | -0.3456 | -0.3527 | -0.3570 | -0.3598 | -0.3633 | -0.3654 |
| **4.45** | 0.0546 | 0.0525 | 0.0273 | -0.0072 | -0.0442 | -0.0800 | -0.1420 | -0.1889 | -0.2229 | -0.2477 | -0.2659 | -0.2904 | -0.3210 | -0.3357 | -0.3500 | -0.3571 | -0.3613 | -0.3641 | -0.3676 | -0.3696 |
| **4.50** | 0.0540 | 0.0509 | 0.0244 | -0.0112 | -0.0491 | -0.0855 | -0.1480 | -0.1949 | -0.2288 | -0.2532 | -0.2712 | -0.2954 | -0.3256 | -0.3401 | -0.3543 | -0.3613 | -0.3654 | -0.3682 | -0.3717 | -0.3737 |

## (A.3) Force-extension relation of a free semiflexible polymer with different persistence lengths $l_P$ and forces F

| | persistence length $l_P/L$ | | | | | | | | | | | | | | | | | | | |
|---|---|---|---|---|---|---|---|---|---|---|---|---|---|---|---|---|---|---|---|---|
| **$\|F\|/F_c$** | **0.1** | **0.2** | **0.3** | **0.4** | **0.5** | **0.6** | **0.8** | **1.0** | **1.2** | **1.4** | **1.6** | **2.0** | **3.0** | **4.0** | **6.0** | **8.0** | **10.0** | **12.0** | **16.0** | **20.0** |
| **0.00** | 0.0000 | -0.0001 | -0.0001 | -0.0001 | -0.0001 | -0.0002 | -0.0002 | -0.0002 | -0.0002 | -0.0002 | -0.0002 | -0.0002 | -0.0002 | -0.0002 | -0.0002 | -0.0002 | -0.0002 | -0.0002 | -0.0002 | -0.0002 |
| **0.05** | -0.0006 | -0.0021 | -0.0041 | -0.0064 | -0.0089 | -0.0116 | -0.0171 | -0.0229 | -0.0287 | -0.0347 | -0.0407 | -0.0527 | -0.0830 | -0.1131 | -0.1726 | -0.2303 | -0.2857 | -0.3382 | -0.4338 | -0.5159 |
| **0.10** | -0.0012 | -0.0040 | -0.0080 | -0.0126 | -0.0176 | -0.0229 | -0.0340 | -0.0455 | -0.0572 | -0.0690 | -0.0809 | -0.1047 | -0.1638 | -0.2215 | -0.3297 | -0.4259 | -0.5087 | -0.5783 | -0.6830 | -0.7530 |
| **0.15** | -0.0017 | -0.0060 | -0.0119 | -0.0189 | -0.0264 | -0.0343 | -0.0509 | -0.0681 | -0.0855 | -0.1030 | -0.1206 | -0.1557 | -0.2412 | -0.3215 | -0.4616 | -0.5720 | -0.6553 | -0.7169 | -0.7966 | -0.8427 |
| **0.20** | -0.0023 | -0.0080 | -0.0159 | -0.0251 | -0.0351 | -0.0457 | -0.0677 | -0.0905 | -0.1135 | -0.1366 | -0.1597 | -0.2053 | -0.3137 | -0.4108 | -0.5657 | -0.6729 | -0.7447 | -0.7932 | -0.8512 | -0.8837 |
| **0.25** | -0.0028 | -0.0100 | -0.0198 | -0.0313 | -0.0439 | -0.0570 | -0.0845 | -0.1127 | -0.1412 | -0.1697 | -0.1979 | -0.2531 | -0.3803 | -0.4881 | -0.6448 | -0.7407 | -0.7996 | -0.8374 | -0.8818 | -0.9069 |
| **0.30** | -0.0034 | -0.0119 | -0.0238 | -0.0376 | -0.0526 | -0.0683 | -0.1011 | -0.1347 | -0.1685 | -0.2020 | -0.2350 | -0.2988 | -0.4407 | -0.5537 | -0.7036 | -0.7866 | -0.8348 | -0.8652 | -0.9012 | -0.9218 |
| **0.35** | -0.0039 | -0.0139 | -0.0277 | -0.0438 | -0.0613 | -0.0796 | -0.1177 | -0.1565 | -0.1953 | -0.2335 | -0.2709 | -0.3422 | -0.4945 | -0.6084 | -0.7474 | -0.8185 | -0.8588 | -0.8842 | -0.9146 | -0.9323 |
| **0.40** | -0.0045 | -0.0159 | -0.0316 | -0.0500 | -0.0699 | -0.0908 | -0.1341 | -0.1780 | -0.2216 | -0.2642 | -0.3055 | -0.3830 | -0.5421 | -0.6537 | -0.7802 | -0.8416 | -0.8761 | -0.8980 | -0.9245 | -0.9401 |
| **0.45** | -0.0050 | -0.0179 | -0.0356 | -0.0562 | -0.0786 | -0.1020 | -0.1503 | -0.1991 | -0.2472 | -0.2939 | -0.3386 | -0.4212 | -0.5837 | -0.6909 | -0.8052 | -0.8589 | -0.8892 | -0.9086 | -0.9322 | -0.9461 |
| **0.50** | -0.0056 | -0.0198 | -0.0395 | -0.0624 | -0.0872 | -0.1131 | -0.1664 | -0.2199 | -0.2722 | -0.3225 | -0.3702 | -0.4568 | -0.6200 | -0.7215 | -0.8247 | -0.8724 | -0.8994 | -0.9169 | -0.9382 | -0.9509 |
| **0.55** | -0.0062 | -0.0218 | -0.0434 | -0.0686 | -0.0958 | -0.1242 | -0.1824 | -0.2403 | -0.2966 | -0.3501 | -0.4003 | -0.4897 | -0.6515 | -0.7468 | -0.8403 | -0.8832 | -0.9077 | -0.9236 | -0.9432 | -0.9548 |
| **0.60** | -0.0067 | -0.0238 | -0.0474 | -0.0748 | -0.1043 | -0.1352 | -0.1981 | -0.2603 | -0.3201 | -0.3765 | -0.4287 | -0.5201 | -0.6787 | -0.7678 | -0.8529 | -0.8920 | -0.9145 | -0.9292 | -0.9473 | -0.9580 |
| **0.65** | -0.0073 | -0.0258 | -0.0513 | -0.0809 | -0.1129 | -0.1461 | -0.2136 | -0.2799 | -0.3430 | -0.4017 | -0.4556 | -0.5481 | -0.7023 | -0.7854 | -0.8634 | -0.8994 | -0.9203 | -0.9339 | -0.9508 | -0.9607 |
| **0.70** | -0.0078 | -0.0277 | -0.0552 | -0.0871 | -0.1214 | -0.1569 | -0.2289 | -0.2990 | -0.3650 | -0.4258 | -0.4809 | -0.5736 | -0.7228 | -0.8003 | -0.8722 | -0.9057 | -0.9252 | -0.9379 | -0.9537 | -0.9631 |
| **0.75** | -0.0084 | -0.0297 | -0.0591 | -0.0932 | -0.1298 | -0.1677 | -0.2440 | -0.3176 | -0.3863 | -0.4488 | -0.5046 | -0.5970 | -0.7405 | -0.8129 | -0.8798 | -0.9111 | -0.9294 | -0.9414 | -0.9563 | -0.9651 |
| **0.80** | -0.0089 | -0.0317 | -0.0630 | -0.0993 | -0.1382 | -0.1784 | -0.2588 | -0.3357 | -0.4067 | -0.4705 | -0.5269 | -0.6184 | -0.7561 | -0.8238 | -0.8863 | -0.9158 | -0.9331 | -0.9445 | -0.9585 | -0.9669 |
| **0.85** | -0.0095 | -0.0337 | -0.0669 | -0.1054 | -0.1466 | -0.1890 | -0.2734 | -0.3534 | -0.4264 | -0.4912 | -0.5477 | -0.6379 | -0.7697 | -0.8333 | -0.8921 | -0.9199 | -0.9363 | -0.9471 | -0.9605 | -0.9685 |
| **0.90** | -0.0100 | -0.0356 | -0.0708 | -0.1115 | -0.1549 | -0.1994 | -0.2877 | -0.3705 | -0.4452 | -0.5107 | -0.5671 | -0.6557 | -0.7817 | -0.8416 | -0.8971 | -0.9236 | -0.9392 | -0.9495 | -0.9623 | -0.9699 |

| | | | | | | | | | | | | | | | | | | | | |
|---|---|---|---|---|---|---|---|---|---|---|---|---|---|---|---|---|---|---|---|---|
| **0.95** | -0.0106 | -0.0376 | -0.0747 | -0.1175 | -0.1632 | -0.2098 | -0.3017 | -0.3871 | -0.4632 | -0.5292 | -0.5853 | -0.6719 | -0.7923 | -0.8489 | -0.9016 | -0.9269 | -0.9418 | -0.9517 | -0.9639 | -0.9712 |
| **1.00** | -0.0111 | -0.0396 | -0.0786 | -0.1236 | -0.1714 | -0.2201 | -0.3155 | -0.4032 | -0.4805 | -0.5466 | -0.6021 | -0.6867 | -0.8018 | -0.8554 | -0.9057 | -0.9298 | -0.9441 | -0.9536 | -0.9653 | -0.9723 |
| **1.05** | -0.0117 | -0.0415 | -0.0825 | -0.1296 | -0.1795 | -0.2303 | -0.3290 | -0.4188 | -0.4969 | -0.5630 | -0.6179 | -0.7002 | -0.8102 | -0.8613 | -0.9093 | -0.9325 | -0.9462 | -0.9553 | -0.9666 | -0.9733 |
| **1.10** | -0.0123 | -0.0435 | -0.0864 | -0.1356 | -0.1877 | -0.2404 | -0.3422 | -0.4339 | -0.5127 | -0.5785 | -0.6325 | -0.7125 | -0.8178 | -0.8666 | -0.9126 | -0.9349 | -0.9482 | -0.9569 | -0.9678 | -0.9743 |
| **1.15** | -0.0128 | -0.0455 | -0.0902 | -0.1415 | -0.1957 | -0.2504 | -0.3551 | -0.4484 | -0.5276 | -0.5930 | -0.6461 | -0.7238 | -0.8247 | -0.8714 | -0.9156 | -0.9372 | -0.9499 | -0.9584 | -0.9689 | -0.9751 |
| **1.20** | -0.0134 | -0.0474 | -0.0941 | -0.1475 | -0.2037 | -0.2602 | -0.3678 | -0.4625 | -0.5419 | -0.6067 | -0.6588 | -0.7341 | -0.8310 | -0.8757 | -0.9184 | -0.9392 | -0.9515 | -0.9597 | -0.9699 | -0.9759 |
| **1.25** | -0.0139 | -0.0494 | -0.0980 | -0.1534 | -0.2116 | -0.2699 | -0.3801 | -0.4760 | -0.5555 | -0.6196 | -0.6706 | -0.7436 | -0.8367 | -0.8797 | -0.9209 | -0.9411 | -0.9530 | -0.9609 | -0.9708 | -0.9766 |
| **1.30** | -0.0145 | -0.0514 | -0.1018 | -0.1593 | -0.2195 | -0.2795 | -0.3922 | -0.4891 | -0.5684 | -0.6317 | -0.6816 | -0.7524 | -0.8419 | -0.8834 | -0.9233 | -0.9428 | -0.9544 | -0.9621 | -0.9716 | -0.9773 |
| **1.35** | -0.0150 | -0.0533 | -0.1057 | -0.1652 | -0.2273 | -0.2890 | -0.4039 | -0.5016 | -0.5807 | -0.6431 | -0.6919 | -0.7604 | -0.8467 | -0.8868 | -0.9255 | -0.9444 | -0.9557 | -0.9631 | -0.9724 | -0.9780 |
| **1.40** | -0.0156 | -0.0553 | -0.1095 | -0.1710 | -0.2350 | -0.2984 | -0.4154 | -0.5137 | -0.5924 | -0.6538 | -0.7015 | -0.7679 | -0.8511 | -0.8900 | -0.9275 | -0.9459 | -0.9568 | -0.9641 | -0.9731 | -0.9785 |
| **1.45** | -0.0161 | -0.0573 | -0.1133 | -0.1768 | -0.2427 | -0.3076 | -0.4266 | -0.5254 | -0.6035 | -0.6639 | -0.7104 | -0.7748 | -0.8553 | -0.8929 | -0.9294 | -0.9473 | -0.9579 | -0.9650 | -0.9738 | -0.9791 |
| **1.50** | -0.0167 | -0.0592 | -0.1171 | -0.1826 | -0.2503 | -0.3167 | -0.4374 | -0.5366 | -0.6141 | -0.6734 | -0.7188 | -0.7812 | -0.8591 | -0.8956 | -0.9311 | -0.9486 | -0.9590 | -0.9659 | -0.9745 | -0.9796 |
| **1.55** | -0.0173 | -0.0612 | -0.1209 | -0.1884 | -0.2578 | -0.3256 | -0.4480 | -0.5473 | -0.6241 | -0.6824 | -0.7266 | -0.7871 | -0.8626 | -0.8982 | -0.9328 | -0.9498 | -0.9600 | -0.9667 | -0.9751 | -0.9801 |
| **1.60** | -0.0178 | -0.0631 | -0.1247 | -0.1941 | -0.2653 | -0.3345 | -0.4583 | -0.5577 | -0.6337 | -0.6908 | -0.7339 | -0.7927 | -0.8660 | -0.9006 | -0.9344 | -0.9510 | -0.9609 | -0.9674 | -0.9756 | -0.9805 |
| **1.65** | -0.0184 | -0.0651 | -0.1285 | -0.1998 | -0.2727 | -0.3432 | -0.4684 | -0.5676 | -0.6427 | -0.6987 | -0.7407 | -0.7979 | -0.8691 | -0.9029 | -0.9358 | -0.9521 | -0.9617 | -0.9682 | -0.9762 | -0.9809 |
| **1.70** | -0.0189 | -0.0670 | -0.1323 | -0.2054 | -0.2800 | -0.3517 | -0.4781 | -0.5772 | -0.6513 | -0.7062 | -0.7472 | -0.8027 | -0.8720 | -0.9050 | -0.9372 | -0.9531 | -0.9625 | -0.9688 | -0.9767 | -0.9813 |
| **1.75** | -0.0195 | -0.0690 | -0.1361 | -0.2111 | -0.2872 | -0.3602 | -0.4876 | -0.5863 | -0.6595 | -0.7133 | -0.7532 | -0.8073 | -0.8748 | -0.9070 | -0.9385 | -0.9540 | -0.9633 | -0.9695 | -0.9771 | -0.9817 |
| **1.80** | -0.0200 | -0.0709 | -0.1399 | -0.2166 | -0.2944 | -0.3685 | -0.4968 | -0.5951 | -0.6673 | -0.7200 | -0.7590 | -0.8116 | -0.8774 | -0.9089 | -0.9397 | -0.9550 | -0.9640 | -0.9701 | -0.9776 | -0.9821 |
| **1.85** | -0.0206 | -0.0729 | -0.1436 | -0.2222 | -0.3014 | -0.3766 | -0.5058 | -0.6035 | -0.6747 | -0.7263 | -0.7643 | -0.8156 | -0.8799 | -0.9107 | -0.9409 | -0.9558 | -0.9647 | -0.9706 | -0.9780 | -0.9824 |
| **1.90** | -0.0211 | -0.0748 | -0.1474 | -0.2277 | -0.3084 | -0.3846 | -0.5144 | -0.6116 | -0.6817 | -0.7323 | -0.7694 | -0.8194 | -0.8822 | -0.9124 | -0.9420 | -0.9567 | -0.9654 | -0.9712 | -0.9784 | -0.9828 |
| **1.95** | -0.0217 | -0.0768 | -0.1511 | -0.2332 | -0.3154 | -0.3925 | -0.5229 | -0.6194 | -0.6884 | -0.7379 | -0.7742 | -0.8230 | -0.8845 | -0.9140 | -0.9431 | -0.9574 | -0.9660 | -0.9717 | -0.9788 | -0.9831 |
| **2.00** | -0.0222 | -0.0787 | -0.1548 | -0.2387 | -0.3222 | -0.4003 | -0.5311 | -0.6269 | -0.6948 | -0.7433 | -0.7788 | -0.8264 | -0.8866 | -0.9156 | -0.9441 | -0.9582 | -0.9666 | -0.9722 | -0.9792 | -0.9834 |
| **2.05** | -0.0228 | -0.0807 | -0.1585 | -0.2441 | -0.3290 | -0.4079 | -0.5390 | -0.6341 | -0.7009 | -0.7484 | -0.7831 | -0.8297 | -0.8886 | -0.9170 | -0.9450 | -0.9589 | -0.9672 | -0.9727 | -0.9795 | -0.9836 |
| **2.10** | -0.0234 | -0.0826 | -0.1622 | -0.2495 | -0.3357 | -0.4154 | -0.5467 | -0.6410 | -0.7067 | -0.7532 | -0.7872 | -0.8328 | -0.8905 | -0.9184 | -0.9460 | -0.9596 | -0.9677 | -0.9731 | -0.9799 | -0.9839 |
| **2.15** | -0.0239 | -0.0846 | -0.1659 | -0.2548 | -0.3423 | -0.4227 | -0.5542 | -0.6476 | -0.7123 | -0.7579 | -0.7910 | -0.8357 | -0.8923 | -0.9198 | -0.9468 | -0.9602 | -0.9682 | -0.9736 | -0.9802 | -0.9842 |
| **2.20** | -0.0245 | -0.0865 | -0.1696 | -0.2601 | -0.3488 | -0.4299 | -0.5614 | -0.6539 | -0.7176 | -0.7623 | -0.7947 | -0.8385 | -0.8941 | -0.9211 | -0.9477 | -0.9609 | -0.9687 | -0.9740 | -0.9805 | -0.9844 |
| **2.25** | -0.0250 | -0.0885 | -0.1732 | -0.2654 | -0.3552 | -0.4370 | -0.5685 | -0.6600 | -0.7226 | -0.7664 | -0.7983 | -0.8411 | -0.8957 | -0.9223 | -0.9485 | -0.9615 | -0.9692 | -0.9744 | -0.9808 | -0.9847 |
| **2.30** | -0.0256 | -0.0904 | -0.1769 | -0.2706 | -0.3616 | -0.4440 | -0.5753 | -0.6659 | -0.7275 | -0.7704 | -0.8016 | -0.8437 | -0.8974 | -0.9235 | -0.9493 | -0.9620 | -0.9697 | -0.9748 | -0.9811 | -0.9849 |
| **2.35** | -0.0261 | -0.0923 | -0.1805 | -0.2758 | -0.3679 | -0.4508 | -0.5819 | -0.6715 | -0.7321 | -0.7743 | -0.8048 | -0.8461 | -0.8989 | -0.9246 | -0.9500 | -0.9626 | -0.9701 | -0.9751 | -0.9814 | -0.9851 |
| **2.40** | -0.0267 | -0.0943 | -0.1842 | -0.2810 | -0.3741 | -0.4575 | -0.5883 | -0.6770 | -0.7365 | -0.7779 | -0.8079 | -0.8485 | -0.9004 | -0.9257 | -0.9507 | -0.9631 | -0.9705 | -0.9755 | -0.9816 | -0.9853 |
| **2.45** | -0.0272 | -0.0962 | -0.1878 | -0.2861 | -0.3802 | -0.4641 | -0.5946 | -0.6822 | -0.7408 | -0.7814 | -0.8109 | -0.8507 | -0.9018 | -0.9267 | -0.9514 | -0.9636 | -0.9709 | -0.9758 | -0.9819 | -0.9855 |
| **2.50** | -0.0278 | -0.0981 | -0.1914 | -0.2912 | -0.3862 | -0.4705 | -0.6006 | -0.6872 | -0.7449 | -0.7847 | -0.8137 | -0.8528 | -0.9032 | -0.9278 | -0.9521 | -0.9641 | -0.9713 | -0.9761 | -0.9821 | -0.9857 |
| **2.55** | -0.0283 | -0.1000 | -0.1950 | -0.2962 | -0.3922 | -0.4768 | -0.6065 | -0.6920 | -0.7488 | -0.7880 | -0.8164 | -0.8549 | -0.9045 | -0.9287 | -0.9527 | -0.9646 | -0.9717 | -0.9765 | -0.9824 | -0.9859 |
| **2.60** | -0.0289 | -0.1020 | -0.1985 | -0.3012 | -0.3981 | -0.4830 | -0.6121 | -0.6967 | -0.7525 | -0.7910 | -0.8190 | -0.8569 | -0.9057 | -0.9297 | -0.9533 | -0.9651 | -0.9721 | -0.9768 | -0.9826 | -0.9861 |
| **2.65** | -0.0294 | -0.1039 | -0.2021 | -0.3061 | -0.4039 | -0.4891 | -0.6176 | -0.7012 | -0.7561 | -0.7940 | -0.8215 | -0.8588 | -0.9070 | -0.9306 | -0.9539 | -0.9655 | -0.9724 | -0.9771 | -0.9828 | -0.9863 |
| **2.70** | -0.0300 | -0.1058 | -0.2057 | -0.3110 | -0.4096 | -0.4950 | -0.6230 | -0.7055 | -0.7596 | -0.7968 | -0.8239 | -0.8606 | -0.9081 | -0.9314 | -0.9545 | -0.9659 | -0.9728 | -0.9773 | -0.9830 | -0.9864 |
| **2.75** | -0.0306 | -0.1077 | -0.2092 | -0.3159 | -0.4152 | -0.5008 | -0.6282 | -0.7097 | -0.7629 | -0.7996 | -0.8262 | -0.8624 | -0.9093 | -0.9323 | -0.9550 | -0.9663 | -0.9731 | -0.9776 | -0.9832 | -0.9866 |

| | | | | | | | | | | | | | | | | | | | | |
|---|---|---|---|---|---|---|---|---|---|---|---|---|---|---|---|---|---|---|---|---|
| **2.80** | -0.0311 | -0.1096 | -0.2127 | -0.3207 | -0.4208 | -0.5066 | -0.6332 | -0.7137 | -0.7661 | -0.8022 | -0.8284 | -0.8641 | -0.9104 | -0.9331 | -0.9556 | -0.9667 | -0.9734 | -0.9779 | -0.9834 | -0.9867 |
| **2.85** | -0.0317 | -0.1116 | -0.2162 | -0.3255 | -0.4262 | -0.5122 | -0.6381 | -0.7176 | -0.7692 | -0.8048 | -0.8306 | -0.8658 | -0.9115 | -0.9339 | -0.9561 | -0.9671 | -0.9737 | -0.9781 | -0.9836 | -0.9869 |
| **2.90** | -0.0322 | -0.1135 | -0.2197 | -0.3303 | -0.4316 | -0.5176 | -0.6428 | -0.7214 | -0.7722 | -0.8072 | -0.8327 | -0.8674 | -0.9125 | -0.9346 | -0.9566 | -0.9675 | -0.9740 | -0.9784 | -0.9838 | -0.9870 |
| **2.95** | -0.0328 | -0.1154 | -0.2232 | -0.3350 | -0.4370 | -0.5230 | -0.6474 | -0.7250 | -0.7751 | -0.8096 | -0.8347 | -0.8690 | -0.9135 | -0.9354 | -0.9571 | -0.9679 | -0.9743 | -0.9786 | -0.9840 | -0.9872 |
| **3.00** | -0.0333 | -0.1173 | -0.2267 | -0.3396 | -0.4422 | -0.5283 | -0.6519 | -0.7285 | -0.7779 | -0.8119 | -0.8366 | -0.8705 | -0.9145 | -0.9361 | -0.9576 | -0.9682 | -0.9746 | -0.9789 | -0.9842 | -0.9873 |
| **3.05** | -0.0339 | -0.1192 | -0.2301 | -0.3443 | -0.4474 | -0.5334 | -0.6562 | -0.7319 | -0.7806 | -0.8141 | -0.8385 | -0.8719 | -0.9154 | -0.9368 | -0.9580 | -0.9686 | -0.9749 | -0.9791 | -0.9843 | -0.9875 |
| **3.10** | -0.0344 | -0.1211 | -0.2336 | -0.3488 | -0.4525 | -0.5385 | -0.6604 | -0.7352 | -0.7832 | -0.8162 | -0.8403 | -0.8733 | -0.9163 | -0.9375 | -0.9585 | -0.9689 | -0.9751 | -0.9793 | -0.9845 | -0.9876 |
| **3.15** | -0.0350 | -0.1230 | -0.2370 | -0.3534 | -0.4575 | -0.5435 | -0.6645 | -0.7383 | -0.7857 | -0.8183 | -0.8421 | -0.8747 | -0.9172 | -0.9381 | -0.9589 | -0.9692 | -0.9754 | -0.9795 | -0.9847 | -0.9877 |
| **3.20** | -0.0355 | -0.1249 | -0.2404 | -0.3579 | -0.4624 | -0.5483 | -0.6685 | -0.7414 | -0.7881 | -0.8203 | -0.8438 | -0.8760 | -0.9181 | -0.9388 | -0.9593 | -0.9695 | -0.9757 | -0.9797 | -0.9848 | -0.9879 |
| **3.25** | -0.0361 | -0.1268 | -0.2438 | -0.3623 | -0.4673 | -0.5531 | -0.6723 | -0.7444 | -0.7905 | -0.8222 | -0.8455 | -0.8773 | -0.9189 | -0.9394 | -0.9597 | -0.9698 | -0.9759 | -0.9799 | -0.9850 | -0.9880 |
| **3.30** | -0.0366 | -0.1287 | -0.2472 | -0.3667 | -0.4721 | -0.5577 | -0.6761 | -0.7473 | -0.7928 | -0.8241 | -0.8471 | -0.8786 | -0.9197 | -0.9400 | -0.9601 | -0.9701 | -0.9761 | -0.9801 | -0.9851 | -0.9881 |
| **3.35** | -0.0372 | -0.1306 | -0.2505 | -0.3711 | -0.4768 | -0.5623 | -0.6797 | -0.7501 | -0.7950 | -0.8260 | -0.8486 | -0.8798 | -0.9205 | -0.9406 | -0.9605 | -0.9704 | -0.9764 | -0.9803 | -0.9852 | -0.9882 |
| **3.40** | -0.0377 | -0.1325 | -0.2539 | -0.3754 | -0.4814 | -0.5667 | -0.6833 | -0.7528 | -0.7971 | -0.8277 | -0.8502 | -0.8810 | -0.9213 | -0.9412 | -0.9609 | -0.9707 | -0.9766 | -0.9805 | -0.9854 | -0.9883 |
| **3.45** | -0.0383 | -0.1344 | -0.2572 | -0.3797 | -0.4860 | -0.5711 | -0.6867 | -0.7554 | -0.7992 | -0.8295 | -0.8516 | -0.8821 | -0.9220 | -0.9417 | -0.9613 | -0.9710 | -0.9768 | -0.9807 | -0.9855 | -0.9884 |
| **3.50** | -0.0389 | -0.1362 | -0.2605 | -0.3840 | -0.4905 | -0.5754 | -0.6901 | -0.7580 | -0.8013 | -0.8311 | -0.8531 | -0.8833 | -0.9228 | -0.9423 | -0.9616 | -0.9713 | -0.9770 | -0.9809 | -0.9857 | -0.9885 |
| **3.55** | -0.0394 | -0.1381 | -0.2638 | -0.3882 | -0.4949 | -0.5796 | -0.6933 | -0.7605 | -0.8032 | -0.8328 | -0.8545 | -0.8843 | -0.9235 | -0.9428 | -0.9620 | -0.9715 | -0.9772 | -0.9810 | -0.9858 | -0.9886 |
| **3.60** | -0.0400 | -0.1400 | -0.2671 | -0.3923 | -0.4993 | -0.5837 | -0.6965 | -0.7629 | -0.8051 | -0.8344 | -0.8558 | -0.8854 | -0.9242 | -0.9433 | -0.9623 | -0.9718 | -0.9774 | -0.9812 | -0.9859 | -0.9887 |
| **3.65** | -0.0405 | -0.1419 | -0.2704 | -0.3964 | -0.5036 | -0.5877 | -0.6996 | -0.7652 | -0.8070 | -0.8359 | -0.8572 | -0.8865 | -0.9248 | -0.9438 | -0.9626 | -0.9720 | -0.9776 | -0.9814 | -0.9860 | -0.9888 |
| **3.70** | -0.0411 | -0.1438 | -0.2736 | -0.4005 | -0.5078 | -0.5916 | -0.7026 | -0.7675 | -0.8088 | -0.8374 | -0.8585 | -0.8875 | -0.9255 | -0.9443 | -0.9630 | -0.9723 | -0.9778 | -0.9815 | -0.9862 | -0.9889 |
| **3.75** | -0.0416 | -0.1456 | -0.2769 | -0.4046 | -0.5120 | -0.5955 | -0.7056 | -0.7697 | -0.8106 | -0.8389 | -0.8597 | -0.8885 | -0.9261 | -0.9448 | -0.9633 | -0.9725 | -0.9780 | -0.9817 | -0.9863 | -0.9890 |
| **3.80** | -0.0422 | -0.1475 | -0.2801 | -0.4086 | -0.5161 | -0.5993 | -0.7084 | -0.7719 | -0.8123 | -0.8403 | -0.8610 | -0.8894 | -0.9268 | -0.9452 | -0.9636 | -0.9727 | -0.9782 | -0.9818 | -0.9864 | -0.9891 |
| **3.85** | -0.0427 | -0.1494 | -0.2833 | -0.4125 | -0.5201 | -0.6030 | -0.7112 | -0.7740 | -0.8140 | -0.8417 | -0.8622 | -0.8904 | -0.9274 | -0.9457 | -0.9639 | -0.9730 | -0.9784 | -0.9820 | -0.9865 | -0.9892 |
| **3.90** | -0.0433 | -0.1512 | -0.2865 | -0.4164 | -0.5241 | -0.6066 | -0.7139 | -0.7760 | -0.8156 | -0.8431 | -0.8633 | -0.8913 | -0.9280 | -0.9461 | -0.9642 | -0.9732 | -0.9786 | -0.9821 | -0.9866 | -0.9893 |
| **3.95** | -0.0438 | -0.1531 | -0.2896 | -0.4203 | -0.5280 | -0.6102 | -0.7166 | -0.7780 | -0.8172 | -0.8444 | -0.8645 | -0.8922 | -0.9286 | -0.9466 | -0.9645 | -0.9734 | -0.9787 | -0.9823 | -0.9867 | -0.9894 |
| **4.00** | -0.0444 | -0.1549 | -0.2928 | -0.4241 | -0.5319 | -0.6137 | -0.7192 | -0.7800 | -0.8188 | -0.8457 | -0.8656 | -0.8931 | -0.9292 | -0.9470 | -0.9648 | -0.9736 | -0.9789 | -0.9824 | -0.9868 | -0.9895 |
| **4.05** | -0.0449 | -0.1568 | -0.2959 | -0.4279 | -0.5356 | -0.6171 | -0.7217 | -0.7819 | -0.8203 | -0.8470 | -0.8667 | -0.8939 | -0.9297 | -0.9474 | -0.9650 | -0.9738 | -0.9791 | -0.9826 | -0.9869 | -0.9895 |
| **4.10** | -0.0455 | -0.1586 | -0.2990 | -0.4317 | -0.5394 | -0.6204 | -0.7242 | -0.7838 | -0.8218 | -0.8482 | -0.8678 | -0.8948 | -0.9303 | -0.9478 | -0.9653 | -0.9740 | -0.9792 | -0.9827 | -0.9870 | -0.9896 |
| **4.15** | -0.0460 | -0.1605 | -0.3021 | -0.4354 | -0.5430 | -0.6237 | -0.7266 | -0.7856 | -0.8232 | -0.8494 | -0.8688 | -0.8956 | -0.9308 | -0.9482 | -0.9656 | -0.9742 | -0.9794 | -0.9828 | -0.9871 | -0.9897 |
| **4.20** | -0.0466 | -0.1623 | -0.3052 | -0.4391 | -0.5467 | -0.6269 | -0.7289 | -0.7873 | -0.8246 | -0.8506 | -0.8698 | -0.8964 | -0.9313 | -0.9486 | -0.9658 | -0.9744 | -0.9795 | -0.9830 | -0.9872 | -0.9898 |
| **4.25** | -0.0471 | -0.1642 | -0.3083 | -0.4427 | -0.5502 | -0.6301 | -0.7312 | -0.7891 | -0.8260 | -0.8518 | -0.8708 | -0.8972 | -0.9318 | -0.9490 | -0.9661 | -0.9746 | -0.9797 | -0.9831 | -0.9873 | -0.9899 |
| **4.30** | -0.0477 | -0.1660 | -0.3114 | -0.4463 | -0.5537 | -0.6332 | -0.7335 | -0.7908 | -0.8274 | -0.8529 | -0.8718 | -0.8979 | -0.9323 | -0.9494 | -0.9663 | -0.9748 | -0.9798 | -0.9832 | -0.9874 | -0.9899 |
| **4.35** | -0.0482 | -0.1679 | -0.3144 | -0.4498 | -0.5571 | -0.6362 | -0.7357 | -0.7924 | -0.8287 | -0.8540 | -0.8728 | -0.8987 | -0.9328 | -0.9498 | -0.9666 | -0.9750 | -0.9800 | -0.9833 | -0.9875 | -0.9900 |
| **4.40** | -0.0488 | -0.1697 | -0.3174 | -0.4534 | -0.5605 | -0.6392 | -0.7378 | -0.7940 | -0.8300 | -0.8551 | -0.8737 | -0.8994 | -0.9333 | -0.9501 | -0.9668 | -0.9751 | -0.9801 | -0.9834 | -0.9876 | -0.9901 |
| **4.45** | -0.0493 | -0.1715 | -0.3204 | -0.4568 | -0.5639 | -0.6421 | -0.7399 | -0.7956 | -0.8313 | -0.8562 | -0.8746 | -0.9002 | -0.9338 | -0.9505 | -0.9671 | -0.9753 | -0.9803 | -0.9836 | -0.9877 | -0.9901 |
| **4.50** | -0.0499 | -0.1733 | -0.3234 | -0.4603 | -0.5671 | -0.6450 | -0.7419 | -0.7971 | -0.8325 | -0.8572 | -0.8755 | -0.9009 | -0.9343 | -0.9508 | -0.9673 | -0.9755 | -0.9804 | -0.9837 | -0.9878 | -0.9902 |

# (B) Force-extension relation of pulled semiflexible polymers with different boundary conditions

## (B.1) Force-extension relation of a clamped semiflexible polymer with different persistence lengths $l_P$ and forces F

| | persistence length $l_P/L$ | | | | | | | | | | | | | | | | | | | |
|---|---|---|---|---|---|---|---|---|---|---|---|---|---|---|---|---|---|---|---|---|
| **$\lvert F\rvert/F_c$** | **0.1** | **0.2** | **0.3** | **0.4** | **0.5** | **0.6** | **0.7** | **0.8** | **0.9** | **1.0** | **1.5** | **2.0** | **3.0** | **4.0** | **5.0** | **6.0** | **7.0** | **8.0** | **9.0** | **10.0** |
| **0** | 0.2000 | 0.3930 | 0.5468 | 0.6496 | 0.7156 | 0.7598 | 0.7913 | 0.8150 | 0.8336 | 0.8488 | 0.8960 | 0.9207 | 0.9463 | 0.9594 | 0.9673 | 0.9727 | 0.9765 | 0.9794 | 0.9817 | 0.9835 |
| **1** | 0.2366 | 0.4827 | 0.6485 | 0.7394 | 0.7918 | 0.8258 | 0.8499 | 0.8680 | 0.8823 | 0.8937 | 0.9285 | 0.9461 | 0.9639 | 0.9729 | 0.9783 | 0.9819 | 0.9845 | 0.9864 | 0.9879 | 0.9891 |
| **2** | 0.2723 | 0.5547 | 0.7115 | 0.7870 | 0.8297 | 0.8576 | 0.8776 | 0.8927 | 0.9044 | 0.9138 | 0.9423 | 0.9566 | 0.9710 | 0.9783 | 0.9826 | 0.9855 | 0.9876 | 0.9891 | 0.9903 | 0.9913 |
| **3** | 0.3067 | 0.6104 | 0.7515 | 0.8156 | 0.8523 | 0.8766 | 0.8941 | 0.9072 | 0.9174 | 0.9256 | 0.9503 | 0.9626 | 0.9751 | 0.9813 | 0.9850 | 0.9875 | 0.9893 | 0.9906 | 0.9917 | 0.9925 |
| **4** | 0.3396 | 0.6529 | 0.7785 | 0.8348 | 0.8677 | 0.8895 | 0.9052 | 0.9170 | 0.9261 | 0.9335 | 0.9556 | 0.9666 | 0.9777 | 0.9833 | 0.9866 | 0.9889 | 0.9904 | 0.9916 | 0.9926 | 0.9933 |
| **5** | 0.3709 | 0.6855 | 0.7981 | 0.8489 | 0.8790 | 0.8990 | 0.9133 | 0.9241 | 0.9325 | 0.9392 | 0.9594 | 0.9695 | 0.9797 | 0.9848 | 0.9878 | 0.9898 | 0.9913 | 0.9924 | 0.9932 | 0.9939 |
| **6** | 0.4004 | 0.7109 | 0.8130 | 0.8599 | 0.8877 | 0.9063 | 0.9197 | 0.9297 | 0.9374 | 0.9437 | 0.9624 | 0.9718 | 0.9812 | 0.9859 | 0.9887 | 0.9906 | 0.9919 | 0.9929 | 0.9937 | 0.9943 |
| **7** | 0.4281 | 0.7311 | 0.8249 | 0.8686 | 0.8948 | 0.9122 | 0.9247 | 0.9341 | 0.9414 | 0.9472 | 0.9648 | 0.9736 | 0.9824 | 0.9868 | 0.9894 | 0.9912 | 0.9924 | 0.9934 | 0.9941 | 0.9947 |
| **8** | 0.4539 | 0.7476 | 0.8347 | 0.8759 | 0.9006 | 0.9171 | 0.9289 | 0.9378 | 0.9447 | 0.9502 | 0.9668 | 0.9751 | 0.9834 | 0.9875 | 0.9900 | 0.9917 | 0.9929 | 0.9938 | 0.9945 | 0.9950 |
| **9** | 0.4779 | 0.7612 | 0.8429 | 0.8821 | 0.9056 | 0.9213 | 0.9325 | 0.9409 | 0.9474 | 0.9527 | 0.9684 | 0.9763 | 0.9842 | 0.9882 | 0.9905 | 0.9921 | 0.9932 | 0.9941 | 0.9947 | 0.9953 |
| **10** | 0.5002 | 0.7727 | 0.8500 | 0.8874 | 0.9098 | 0.9248 | 0.9355 | 0.9436 | 0.9498 | 0.9548 | 0.9699 | 0.9774 | 0.9849 | 0.9887 | 0.9910 | 0.9925 | 0.9935 | 0.9943 | 0.9950 | 0.9955 |
| **11** | 0.5208 | 0.7826 | 0.8561 | 0.8920 | 0.9135 | 0.9279 | 0.9382 | 0.9459 | 0.9519 | 0.9567 | 0.9711 | 0.9783 | 0.9855 | 0.9892 | 0.9913 | 0.9928 | 0.9938 | 0.9946 | 0.9952 | 0.9957 |
| **12** | 0.5397 | 0.7912 | 0.8616 | 0.8961 | 0.9168 | 0.9307 | 0.9405 | 0.9480 | 0.9537 | 0.9583 | 0.9722 | 0.9792 | 0.9861 | 0.9896 | 0.9917 | 0.9930 | 0.9940 | 0.9948 | 0.9954 | 0.9958 |
| **13** | 0.5573 | 0.7989 | 0.8664 | 0.8997 | 0.9197 | 0.9331 | 0.9426 | 0.9498 | 0.9554 | 0.9598 | 0.9732 | 0.9799 | 0.9866 | 0.9899 | 0.9920 | 0.9933 | 0.9943 | 0.9950 | 0.9955 | 0.9960 |
| **14** | 0.5734 | 0.8056 | 0.8708 | 0.9030 | 0.9224 | 0.9353 | 0.9445 | 0.9514 | 0.9568 | 0.9611 | 0.9741 | 0.9806 | 0.9870 | 0.9903 | 0.9922 | 0.9935 | 0.9944 | 0.9951 | 0.9957 | 0.9961 |
| **15** | 0.5883 | 0.8117 | 0.8748 | 0.9060 | 0.9248 | 0.9373 | 0.9462 | 0.9529 | 0.9582 | 0.9623 | 0.9749 | 0.9812 | 0.9874 | 0.9906 | 0.9925 | 0.9937 | 0.9946 | 0.9953 | 0.9958 | 0.9962 |
| **16** | 0.6020 | 0.8173 | 0.8784 | 0.9087 | 0.9269 | 0.9391 | 0.9478 | 0.9543 | 0.9594 | 0.9634 | 0.9756 | 0.9817 | 0.9878 | 0.9908 | 0.9927 | 0.9939 | 0.9948 | 0.9954 | 0.9959 | 0.9963 |
| **17** | 0.6147 | 0.8223 | 0.8817 | 0.9112 | 0.9289 | 0.9407 | 0.9492 | 0.9555 | 0.9605 | 0.9644 | 0.9763 | 0.9822 | 0.9881 | 0.9911 | 0.9929 | 0.9941 | 0.9949 | 0.9955 | 0.9960 | 0.9964 |
| **18** | 0.6264 | 0.8269 | 0.8847 | 0.9135 | 0.9307 | 0.9423 | 0.9505 | 0.9567 | 0.9615 | 0.9653 | 0.9769 | 0.9827 | 0.9884 | 0.9913 | 0.9931 | 0.9942 | 0.9950 | 0.9957 | 0.9961 | 0.9965 |
| **19** | 0.6373 | 0.8312 | 0.8875 | 0.9156 | 0.9324 | 0.9437 | 0.9517 | 0.9577 | 0.9624 | 0.9662 | 0.9775 | 0.9831 | 0.9887 | 0.9915 | 0.9932 | 0.9944 | 0.9952 | 0.9958 | 0.9962 | 0.9966 |
| **20** | 0.6474 | 0.8351 | 0.8901 | 0.9175 | 0.9340 | 0.9450 | 0.9528 | 0.9587 | 0.9633 | 0.9670 | 0.9780 | 0.9835 | 0.9890 | 0.9917 | 0.9934 | 0.9945 | 0.9953 | 0.9959 | 0.9963 | 0.9967 |
| **21** | 0.6567 | 0.8388 | 0.8926 | 0.9194 | 0.9355 | 0.9462 | 0.9539 | 0.9596 | 0.9641 | 0.9677 | 0.9785 | 0.9838 | 0.9892 | 0.9919 | 0.9935 | 0.9946 | 0.9954 | 0.9960 | 0.9964 | 0.9968 |
| **22** | 0.6654 | 0.8423 | 0.8948 | 0.9211 | 0.9368 | 0.9474 | 0.9549 | 0.9605 | 0.9649 | 0.9684 | 0.9789 | 0.9842 | 0.9895 | 0.9921 | 0.9937 | 0.9947 | 0.9955 | 0.9960 | 0.9965 | 0.9968 |
| **23** | 0.6735 | 0.8455 | 0.8970 | 0.9227 | 0.9381 | 0.9484 | 0.9558 | 0.9613 | 0.9656 | 0.9690 | 0.9794 | 0.9845 | 0.9897 | 0.9923 | 0.9938 | 0.9948 | 0.9956 | 0.9961 | 0.9966 | 0.9969 |
| **24** | 0.6811 | 0.8485 | 0.8990 | 0.9242 | 0.9393 | 0.9494 | 0.9567 | 0.9621 | 0.9663 | 0.9696 | 0.9798 | 0.9848 | 0.9899 | 0.9924 | 0.9939 | 0.9949 | 0.9957 | 0.9962 | 0.9966 | 0.9970 |
| **25** | 0.6882 | 0.8513 | 0.9009 | 0.9256 | 0.9405 | 0.9504 | 0.9575 | 0.9628 | 0.9669 | 0.9702 | 0.9801 | 0.9851 | 0.9901 | 0.9926 | 0.9940 | 0.9950 | 0.9957 | 0.9963 | 0.9967 | 0.9970 |
| **26** | 0.6948 | 0.8540 | 0.9027 | 0.9270 | 0.9416 | 0.9513 | 0.9582 | 0.9635 | 0.9675 | 0.9708 | 0.9805 | 0.9854 | 0.9902 | 0.9927 | 0.9941 | 0.9951 | 0.9958 | 0.9963 | 0.9967 | 0.9971 |
| **27** | 0.7011 | 0.8566 | 0.9043 | 0.9282 | 0.9426 | 0.9521 | 0.9590 | 0.9641 | 0.9681 | 0.9713 | 0.9808 | 0.9856 | 0.9904 | 0.9928 | 0.9943 | 0.9952 | 0.9959 | 0.9964 | 0.9968 | 0.9971 |
| **28** | 0.7069 | 0.8590 | 0.9060 | 0.9294 | 0.9435 | 0.9529 | 0.9597 | 0.9647 | 0.9686 | 0.9718 | 0.9812 | 0.9859 | 0.9906 | 0.9929 | 0.9943 | 0.9953 | 0.9960 | 0.9965 | 0.9969 | 0.9972 |
| **29** | 0.7125 | 0.8613 | 0.9075 | 0.9306 | 0.9445 | 0.9537 | 0.9603 | 0.9653 | 0.9691 | 0.9722 | 0.9815 | 0.9861 | 0.9907 | 0.9930 | 0.9944 | 0.9954 | 0.9960 | 0.9965 | 0.9969 | 0.9972 |

| | | | | | | | | | | | | | | | | | | | | |
|---|---|---|---|---|---|---|---|---|---|---|---|---|---|---|---|---|---|---|---|---|
| **30** | 0.7177 | 0.8634 | 0.9089 | 0.9317 | 0.9453 | 0.9544 | 0.9609 | 0.9658 | 0.9696 | 0.9726 | 0.9818 | 0.9863 | 0.9909 | 0.9932 | 0.9945 | 0.9954 | 0.9961 | 0.9966 | 0.9970 | 0.9973 |
| **31** | 0.7226 | 0.8655 | 0.9103 | 0.9327 | 0.9462 | 0.9551 | 0.9615 | 0.9663 | 0.9701 | 0.9731 | 0.9820 | 0.9865 | 0.9910 | 0.9933 | 0.9946 | 0.9955 | 0.9962 | 0.9966 | 0.9970 | 0.9973 |
| **32** | 0.7273 | 0.8675 | 0.9116 | 0.9337 | 0.9470 | 0.9558 | 0.9621 | 0.9668 | 0.9705 | 0.9735 | 0.9823 | 0.9867 | 0.9912 | 0.9934 | 0.9947 | 0.9956 | 0.9962 | 0.9967 | 0.9971 | 0.9973 |
| **33** | 0.7317 | 0.8694 | 0.9129 | 0.9347 | 0.9477 | 0.9564 | 0.9626 | 0.9673 | 0.9709 | 0.9738 | 0.9826 | 0.9869 | 0.9913 | 0.9935 | 0.9948 | 0.9956 | 0.9963 | 0.9967 | 0.9971 | 0.9974 |
| **34** | 0.7360 | 0.8712 | 0.9141 | 0.9356 | 0.9484 | 0.9570 | 0.9632 | 0.9678 | 0.9713 | 0.9742 | 0.9828 | 0.9871 | 0.9914 | 0.9935 | 0.9948 | 0.9957 | 0.9963 | 0.9968 | 0.9971 | 0.9974 |
| **35** | 0.7400 | 0.8730 | 0.9153 | 0.9364 | 0.9491 | 0.9576 | 0.9637 | 0.9682 | 0.9717 | 0.9746 | 0.9830 | 0.9873 | 0.9915 | 0.9936 | 0.9949 | 0.9958 | 0.9964 | 0.9968 | 0.9972 | 0.9975 |
| **36** | 0.7438 | 0.8746 | 0.9164 | 0.9373 | 0.9498 | 0.9582 | 0.9641 | 0.9686 | 0.9721 | 0.9749 | 0.9833 | 0.9874 | 0.9916 | 0.9937 | 0.9950 | 0.9958 | 0.9964 | 0.9969 | 0.9972 | 0.9975 |
| **37** | 0.7475 | 0.8762 | 0.9175 | 0.9381 | 0.9505 | 0.9587 | 0.9646 | 0.9690 | 0.9725 | 0.9752 | 0.9835 | 0.9876 | 0.9917 | 0.9938 | 0.9950 | 0.9959 | 0.9965 | 0.9969 | 0.9972 | 0.9975 |
| **38** | 0.7510 | 0.8778 | 0.9185 | 0.9389 | 0.9511 | 0.9592 | 0.9650 | 0.9694 | 0.9728 | 0.9755 | 0.9837 | 0.9878 | 0.9918 | 0.9939 | 0.9951 | 0.9959 | 0.9965 | 0.9969 | 0.9973 | 0.9976 |
| **39** | 0.7543 | 0.8793 | 0.9195 | 0.9396 | 0.9517 | 0.9597 | 0.9655 | 0.9698 | 0.9731 | 0.9758 | 0.9839 | 0.9879 | 0.9919 | 0.9940 | 0.9952 | 0.9960 | 0.9965 | 0.9970 | 0.9973 | 0.9976 |
| **40** | 0.7575 | 0.8807 | 0.9204 | 0.9403 | 0.9522 | 0.9602 | 0.9659 | 0.9701 | 0.9735 | 0.9761 | 0.9841 | 0.9881 | 0.9920 | 0.9940 | 0.9952 | 0.9960 | 0.9966 | 0.9970 | 0.9973 | 0.9976 |
| **41** | 0.7606 | 0.8821 | 0.9214 | 0.9410 | 0.9528 | 0.9607 | 0.9663 | 0.9705 | 0.9738 | 0.9764 | 0.9843 | 0.9882 | 0.9921 | 0.9941 | 0.9953 | 0.9961 | 0.9966 | 0.9970 | 0.9974 | 0.9976 |
| **42** | 0.7635 | 0.8834 | 0.9223 | 0.9417 | 0.9533 | 0.9611 | 0.9667 | 0.9708 | 0.9741 | 0.9767 | 0.9844 | 0.9883 | 0.9922 | 0.9942 | 0.9953 | 0.9961 | 0.9967 | 0.9971 | 0.9974 | 0.9977 |
| **43** | 0.7663 | 0.8847 | 0.9231 | 0.9423 | 0.9539 | 0.9615 | 0.9670 | 0.9711 | 0.9744 | 0.9769 | 0.9846 | 0.9885 | 0.9923 | 0.9942 | 0.9954 | 0.9962 | 0.9967 | 0.9971 | 0.9974 | 0.9977 |
| **44** | 0.7691 | 0.8860 | 0.9239 | 0.9429 | 0.9544 | 0.9620 | 0.9674 | 0.9715 | 0.9746 | 0.9772 | 0.9848 | 0.9886 | 0.9924 | 0.9943 | 0.9954 | 0.9962 | 0.9967 | 0.9971 | 0.9975 | 0.9977 |
| **45** | 0.7717 | 0.8872 | 0.9248 | 0.9436 | 0.9548 | 0.9624 | 0.9677 | 0.9718 | 0.9749 | 0.9774 | 0.9849 | 0.9887 | 0.9925 | 0.9944 | 0.9955 | 0.9962 | 0.9968 | 0.9972 | 0.9975 | 0.9977 |
| **46** | 0.7742 | 0.8883 | 0.9255 | 0.9441 | 0.9553 | 0.9627 | 0.9681 | 0.9721 | 0.9752 | 0.9776 | 0.9851 | 0.9888 | 0.9925 | 0.9944 | 0.9955 | 0.9963 | 0.9968 | 0.9972 | 0.9975 | 0.9978 |
| **47** | 0.7767 | 0.8895 | 0.9263 | 0.9447 | 0.9558 | 0.9631 | 0.9684 | 0.9723 | 0.9754 | 0.9779 | 0.9852 | 0.9889 | 0.9926 | 0.9945 | 0.9956 | 0.9963 | 0.9968 | 0.9972 | 0.9975 | 0.9978 |
| **48** | 0.7790 | 0.8906 | 0.9270 | 0.9453 | 0.9562 | 0.9635 | 0.9687 | 0.9726 | 0.9757 | 0.9781 | 0.9854 | 0.9890 | 0.9927 | 0.9945 | 0.9956 | 0.9963 | 0.9969 | 0.9973 | 0.9976 | 0.9978 |
| **49** | 0.7813 | 0.8916 | 0.9277 | 0.9458 | 0.9566 | 0.9639 | 0.9690 | 0.9729 | 0.9759 | 0.9783 | 0.9855 | 0.9892 | 0.9928 | 0.9946 | 0.9957 | 0.9964 | 0.9969 | 0.9973 | 0.9976 | 0.9978 |
| **50** | 0.7835 | 0.8927 | 0.9284 | 0.9463 | 0.9570 | 0.9642 | 0.9693 | 0.9731 | 0.9761 | 0.9785 | 0.9857 | 0.9893 | 0.9928 | 0.9946 | 0.9957 | 0.9964 | 0.9969 | 0.9973 | 0.9976 | 0.9979 |
| **51** | 0.7857 | 0.8937 | 0.9291 | 0.9468 | 0.9574 | 0.9645 | 0.9696 | 0.9734 | 0.9764 | 0.9787 | 0.9858 | 0.9894 | 0.9929 | 0.9947 | 0.9957 | 0.9965 | 0.9970 | 0.9973 | 0.9976 | 0.9979 |
| **52** | 0.7877 | 0.8946 | 0.9297 | 0.9473 | 0.9578 | 0.9649 | 0.9699 | 0.9736 | 0.9766 | 0.9789 | 0.9859 | 0.9895 | 0.9930 | 0.9947 | 0.9958 | 0.9965 | 0.9970 | 0.9974 | 0.9977 | 0.9979 |
| **53** | 0.7897 | 0.8956 | 0.9304 | 0.9478 | 0.9582 | 0.9652 | 0.9701 | 0.9739 | 0.9768 | 0.9791 | 0.9861 | 0.9895 | 0.9930 | 0.9948 | 0.9958 | 0.9965 | 0.9970 | 0.9974 | 0.9977 | 0.9979 |
| **54** | 0.7917 | 0.8965 | 0.9310 | 0.9482 | 0.9586 | 0.9655 | 0.9704 | 0.9741 | 0.9770 | 0.9793 | 0.9862 | 0.9896 | 0.9931 | 0.9948 | 0.9959 | 0.9965 | 0.9970 | 0.9974 | 0.9977 | 0.9979 |
| **55** | 0.7936 | 0.8974 | 0.9316 | 0.9487 | 0.9589 | 0.9658 | 0.9707 | 0.9743 | 0.9772 | 0.9795 | 0.9863 | 0.9897 | 0.9932 | 0.9949 | 0.9959 | 0.9966 | 0.9971 | 0.9974 | 0.9977 | 0.9979 |
| **56** | 0.7954 | 0.8983 | 0.9322 | 0.9491 | 0.9593 | 0.9661 | 0.9709 | 0.9746 | 0.9774 | 0.9796 | 0.9864 | 0.9898 | 0.9932 | 0.9949 | 0.9959 | 0.9966 | 0.9971 | 0.9975 | 0.9977 | 0.9980 |
| **57** | 0.7972 | 0.8992 | 0.9328 | 0.9496 | 0.9596 | 0.9664 | 0.9712 | 0.9748 | 0.9776 | 0.9798 | 0.9865 | 0.9899 | 0.9933 | 0.9950 | 0.9960 | 0.9966 | 0.9971 | 0.9975 | 0.9978 | 0.9980 |
| **58** | 0.7989 | 0.9000 | 0.9333 | 0.9500 | 0.9600 | 0.9666 | 0.9714 | 0.9750 | 0.9778 | 0.9800 | 0.9867 | 0.9900 | 0.9933 | 0.9950 | 0.9960 | 0.9967 | 0.9971 | 0.9975 | 0.9978 | 0.9980 |
| **59** | 0.8006 | 0.9008 | 0.9339 | 0.9504 | 0.9603 | 0.9669 | 0.9716 | 0.9752 | 0.9779 | 0.9801 | 0.9868 | 0.9901 | 0.9934 | 0.9950 | 0.9960 | 0.9967 | 0.9972 | 0.9975 | 0.9978 | 0.9980 |
| **60** | 0.8023 | 0.9016 | 0.9344 | 0.9508 | 0.9606 | 0.9672 | 0.9719 | 0.9754 | 0.9781 | 0.9803 | 0.9869 | 0.9902 | 0.9934 | 0.9951 | 0.9961 | 0.9967 | 0.9972 | 0.9975 | 0.9978 | 0.9980 |
| **61** | 0.8039 | 0.9024 | 0.9349 | 0.9512 | 0.9609 | 0.9674 | 0.9721 | 0.9756 | 0.9783 | 0.9805 | 0.9870 | 0.9902 | 0.9935 | 0.9951 | 0.9961 | 0.9967 | 0.9972 | 0.9976 | 0.9978 | 0.9980 |
| **62** | 0.8055 | 0.9031 | 0.9354 | 0.9515 | 0.9612 | 0.9677 | 0.9723 | 0.9758 | 0.9785 | 0.9806 | 0.9871 | 0.9903 | 0.9935 | 0.9952 | 0.9961 | 0.9968 | 0.9972 | 0.9976 | 0.9978 | 0.9981 |
| **63** | 0.8070 | 0.9039 | 0.9359 | 0.9519 | 0.9615 | 0.9679 | 0.9725 | 0.9759 | 0.9786 | 0.9808 | 0.9872 | 0.9904 | 0.9936 | 0.9952 | 0.9962 | 0.9968 | 0.9973 | 0.9976 | 0.9979 | 0.9981 |
| **64** | 0.8085 | 0.9046 | 0.9364 | 0.9523 | 0.9618 | 0.9682 | 0.9727 | 0.9761 | 0.9788 | 0.9809 | 0.9873 | 0.9905 | 0.9936 | 0.9952 | 0.9962 | 0.9968 | 0.9973 | 0.9976 | 0.9979 | 0.9981 |
| **65** | 0.8099 | 0.9053 | 0.9368 | 0.9526 | 0.9621 | 0.9684 | 0.9729 | 0.9763 | 0.9789 | 0.9810 | 0.9874 | 0.9905 | 0.9937 | 0.9953 | 0.9962 | 0.9968 | 0.9973 | 0.9976 | 0.9979 | 0.9981 |
| **66** | 0.8113 | 0.9060 | 0.9373 | 0.9530 | 0.9624 | 0.9686 | 0.9731 | 0.9765 | 0.9791 | 0.9812 | 0.9875 | 0.9906 | 0.9937 | 0.9953 | 0.9962 | 0.9969 | 0.9973 | 0.9976 | 0.9979 | 0.9981 |

| | | | | | | | | | | | | | | | | | | | | |
|---|---|---|---|---|---|---|---|---|---|---|---|---|---|---|---|---|---|---|---|---|
| **67** | 0.8127 | 0.9066 | 0.9378 | 0.9533 | 0.9626 | 0.9689 | 0.9733 | 0.9766 | 0.9792 | 0.9813 | 0.9875 | 0.9907 | 0.9938 | 0.9953 | 0.9963 | 0.9969 | 0.9973 | 0.9977 | 0.9979 | 0.9981 |
| **68** | 0.8141 | 0.9073 | 0.9382 | 0.9536 | 0.9629 | 0.9691 | 0.9735 | 0.9768 | 0.9794 | 0.9814 | 0.9876 | 0.9907 | 0.9938 | 0.9954 | 0.9963 | 0.9969 | 0.9973 | 0.9977 | 0.9979 | 0.9981 |
| **69** | 0.8154 | 0.9080 | 0.9386 | 0.9540 | 0.9632 | 0.9693 | 0.9737 | 0.9770 | 0.9795 | 0.9816 | 0.9877 | 0.9908 | 0.9939 | 0.9954 | 0.9963 | 0.9969 | 0.9974 | 0.9977 | 0.9980 | 0.9982 |
| **70** | 0.8167 | 0.9086 | 0.9390 | 0.9543 | 0.9634 | 0.9695 | 0.9739 | 0.9771 | 0.9797 | 0.9817 | 0.9878 | 0.9909 | 0.9939 | 0.9954 | 0.9963 | 0.9970 | 0.9974 | 0.9977 | 0.9980 | 0.9982 |
| **71** | 0.8180 | 0.9092 | 0.9395 | 0.9546 | 0.9637 | 0.9697 | 0.9740 | 0.9773 | 0.9798 | 0.9818 | 0.9879 | 0.9909 | 0.9939 | 0.9955 | 0.9964 | 0.9970 | 0.9974 | 0.9977 | 0.9980 | 0.9982 |
| **72** | 0.8192 | 0.9098 | 0.9399 | 0.9549 | 0.9639 | 0.9699 | 0.9742 | 0.9774 | 0.9799 | 0.9820 | 0.9880 | 0.9910 | 0.9940 | 0.9955 | 0.9964 | 0.9970 | 0.9974 | 0.9977 | 0.9980 | 0.9982 |
| **73** | 0.8204 | 0.9104 | 0.9403 | 0.9552 | 0.9641 | 0.9701 | 0.9744 | 0.9776 | 0.9801 | 0.9821 | 0.9880 | 0.9910 | 0.9940 | 0.9955 | 0.9964 | 0.9970 | 0.9974 | 0.9978 | 0.9980 | 0.9982 |
| **74** | 0.8216 | 0.9110 | 0.9407 | 0.9555 | 0.9644 | 0.9703 | 0.9746 | 0.9777 | 0.9802 | 0.9822 | 0.9881 | 0.9911 | 0.9941 | 0.9955 | 0.9964 | 0.9970 | 0.9975 | 0.9978 | 0.9980 | 0.9982 |
| **75** | 0.8228 | 0.9116 | 0.9410 | 0.9558 | 0.9646 | 0.9705 | 0.9747 | 0.9779 | 0.9803 | 0.9823 | 0.9882 | 0.9912 | 0.9941 | 0.9956 | 0.9965 | 0.9970 | 0.9975 | 0.9978 | 0.9980 | 0.9982 |
| **76** | 0.8239 | 0.9121 | 0.9414 | 0.9560 | 0.9648 | 0.9707 | 0.9749 | 0.9780 | 0.9805 | 0.9824 | 0.9883 | 0.9912 | 0.9941 | 0.9956 | 0.9965 | 0.9971 | 0.9975 | 0.9978 | 0.9980 | 0.9982 |
| **77** | 0.8250 | 0.9127 | 0.9418 | 0.9563 | 0.9651 | 0.9709 | 0.9750 | 0.9782 | 0.9806 | 0.9825 | 0.9883 | 0.9913 | 0.9942 | 0.9956 | 0.9965 | 0.9971 | 0.9975 | 0.9978 | 0.9981 | 0.9983 |
| **78** | 0.8261 | 0.9132 | 0.9421 | 0.9566 | 0.9653 | 0.9711 | 0.9752 | 0.9783 | 0.9807 | 0.9826 | 0.9884 | 0.9913 | 0.9942 | 0.9957 | 0.9965 | 0.9971 | 0.9975 | 0.9978 | 0.9981 | 0.9983 |
| **79** | 0.8272 | 0.9137 | 0.9425 | 0.9569 | 0.9655 | 0.9712 | 0.9753 | 0.9784 | 0.9808 | 0.9827 | 0.9885 | 0.9914 | 0.9942 | 0.9957 | 0.9965 | 0.9971 | 0.9975 | 0.9978 | 0.9981 | 0.9983 |
| **80** | 0.8282 | 0.9143 | 0.9428 | 0.9571 | 0.9657 | 0.9714 | 0.9755 | 0.9786 | 0.9809 | 0.9828 | 0.9886 | 0.9914 | 0.9943 | 0.9957 | 0.9966 | 0.9971 | 0.9975 | 0.9979 | 0.9981 | 0.9983 |
| **81** | 0.8293 | 0.9148 | 0.9432 | 0.9574 | 0.9659 | 0.9716 | 0.9756 | 0.9787 | 0.9811 | 0.9829 | 0.9886 | 0.9915 | 0.9943 | 0.9957 | 0.9966 | 0.9972 | 0.9976 | 0.9979 | 0.9981 | 0.9983 |
| **82** | 0.8303 | 0.9153 | 0.9435 | 0.9576 | 0.9661 | 0.9717 | 0.9758 | 0.9788 | 0.9812 | 0.9830 | 0.9887 | 0.9915 | 0.9943 | 0.9958 | 0.9966 | 0.9972 | 0.9976 | 0.9979 | 0.9981 | 0.9983 |
| **83** | 0.8313 | 0.9158 | 0.9438 | 0.9579 | 0.9663 | 0.9719 | 0.9759 | 0.9789 | 0.9813 | 0.9831 | 0.9888 | 0.9916 | 0.9944 | 0.9958 | 0.9966 | 0.9972 | 0.9976 | 0.9979 | 0.9981 | 0.9983 |
| **84** | 0.8323 | 0.9163 | 0.9442 | 0.9581 | 0.9665 | 0.9721 | 0.9761 | 0.9791 | 0.9814 | 0.9832 | 0.9888 | 0.9916 | 0.9944 | 0.9958 | 0.9966 | 0.9972 | 0.9976 | 0.9979 | 0.9981 | 0.9983 |
| **85** | 0.8332 | 0.9167 | 0.9445 | 0.9584 | 0.9667 | 0.9722 | 0.9762 | 0.9792 | 0.9815 | 0.9833 | 0.9889 | 0.9917 | 0.9944 | 0.9958 | 0.9967 | 0.9972 | 0.9976 | 0.9979 | 0.9981 | 0.9983 |
| **86** | 0.8342 | 0.9172 | 0.9448 | 0.9586 | 0.9669 | 0.9724 | 0.9763 | 0.9793 | 0.9816 | 0.9834 | 0.9890 | 0.9917 | 0.9945 | 0.9959 | 0.9967 | 0.9972 | 0.9976 | 0.9979 | 0.9982 | 0.9983 |
| **87** | 0.8351 | 0.9177 | 0.9451 | 0.9588 | 0.9671 | 0.9725 | 0.9765 | 0.9794 | 0.9817 | 0.9835 | 0.9890 | 0.9918 | 0.9945 | 0.9959 | 0.9967 | 0.9973 | 0.9976 | 0.9979 | 0.9982 | 0.9984 |
| **88** | 0.8360 | 0.9181 | 0.9454 | 0.9590 | 0.9672 | 0.9727 | 0.9766 | 0.9795 | 0.9818 | 0.9836 | 0.9891 | 0.9918 | 0.9945 | 0.9959 | 0.9967 | 0.9973 | 0.9977 | 0.9980 | 0.9982 | 0.9984 |
| **89** | 0.8369 | 0.9186 | 0.9457 | 0.9593 | 0.9674 | 0.9728 | 0.9767 | 0.9796 | 0.9819 | 0.9837 | 0.9891 | 0.9919 | 0.9946 | 0.9959 | 0.9967 | 0.9973 | 0.9977 | 0.9980 | 0.9982 | 0.9984 |
| **90** | 0.8378 | 0.9190 | 0.9460 | 0.9595 | 0.9676 | 0.9730 | 0.9768 | 0.9797 | 0.9820 | 0.9838 | 0.9892 | 0.9919 | 0.9946 | 0.9959 | 0.9968 | 0.9973 | 0.9977 | 0.9980 | 0.9982 | 0.9984 |
| **91** | 0.8387 | 0.9194 | 0.9463 | 0.9597 | 0.9678 | 0.9731 | 0.9770 | 0.9798 | 0.9821 | 0.9839 | 0.9892 | 0.9919 | 0.9946 | 0.9960 | 0.9968 | 0.9973 | 0.9977 | 0.9980 | 0.9982 | 0.9984 |
| **92** | 0.8395 | 0.9198 | 0.9466 | 0.9599 | 0.9679 | 0.9733 | 0.9771 | 0.9800 | 0.9822 | 0.9840 | 0.9893 | 0.9920 | 0.9947 | 0.9960 | 0.9968 | 0.9973 | 0.9977 | 0.9980 | 0.9982 | 0.9984 |
| **93** | 0.8404 | 0.9203 | 0.9468 | 0.9601 | 0.9681 | 0.9734 | 0.9772 | 0.9801 | 0.9823 | 0.9840 | 0.9894 | 0.9920 | 0.9947 | 0.9960 | 0.9968 | 0.9973 | 0.9977 | 0.9980 | 0.9982 | 0.9984 |
| **94** | 0.8412 | 0.9207 | 0.9471 | 0.9603 | 0.9683 | 0.9735 | 0.9773 | 0.9802 | 0.9824 | 0.9841 | 0.9894 | 0.9921 | 0.9947 | 0.9960 | 0.9968 | 0.9974 | 0.9977 | 0.9980 | 0.9982 | 0.9984 |
| **95** | 0.8420 | 0.9211 | 0.9474 | 0.9605 | 0.9684 | 0.9737 | 0.9774 | 0.9803 | 0.9825 | 0.9842 | 0.9895 | 0.9921 | 0.9947 | 0.9961 | 0.9968 | 0.9974 | 0.9977 | 0.9980 | 0.9982 | 0.9984 |
| **96** | 0.8428 | 0.9215 | 0.9476 | 0.9607 | 0.9686 | 0.9738 | 0.9776 | 0.9804 | 0.9825 | 0.9843 | 0.9895 | 0.9921 | 0.9948 | 0.9961 | 0.9969 | 0.9974 | 0.9978 | 0.9980 | 0.9983 | 0.9984 |
| **97** | 0.8436 | 0.9219 | 0.9479 | 0.9609 | 0.9687 | 0.9739 | 0.9777 | 0.9805 | 0.9826 | 0.9844 | 0.9896 | 0.9922 | 0.9948 | 0.9961 | 0.9969 | 0.9974 | 0.9978 | 0.9980 | 0.9983 | 0.9984 |
| **98** | 0.8444 | 0.9222 | 0.9482 | 0.9611 | 0.9689 | 0.9741 | 0.9778 | 0.9806 | 0.9827 | 0.9844 | 0.9896 | 0.9922 | 0.9948 | 0.9961 | 0.9969 | 0.9974 | 0.9978 | 0.9981 | 0.9983 | 0.9984 |
| **99** | 0.8451 | 0.9226 | 0.9484 | 0.9613 | 0.9690 | 0.9742 | 0.9779 | 0.9806 | 0.9828 | 0.9845 | 0.9897 | 0.9923 | 0.9948 | 0.9961 | 0.9969 | 0.9974 | 0.9978 | 0.9981 | 0.9983 | 0.9985 |
| **100** | 0.8459 | 0.9230 | 0.9487 | 0.9615 | 0.9692 | 0.9743 | 0.9780 | 0.9807 | 0.9829 | 0.9846 | 0.9897 | 0.9923 | 0.9949 | 0.9961 | 0.9969 | 0.9974 | 0.9978 | 0.9981 | 0.9983 | 0.9985 |

## (B.2) Force-extension relation of a half-clamped semiflexible polymer with different persistence lengths $l_P$ and forces F

| | persistence length $l_P/L$ | | | | | | | | | | | | | | | | | | | |
|---|---|---|---|---|---|---|---|---|---|---|---|---|---|---|---|---|---|---|---|---|
| $\|F\|/F_c$ | 0.1 | 0.2 | 0.3 | 0.4 | 0.5 | 0.6 | 0.8 | 1.0 | 1.2 | 1.4 | 1.6 | 2.0 | 3.0 | 4.0 | 6.0 | 8.0 | 10.0 | 12.0 | 16.0 | 20.0 |
| 0 | 0.1000 | 0.1987 | 0.2894 | 0.3672 | 0.4324 | 0.4867 | 0.5709 | 0.6322 | 0.6785 | 0.7147 | 0.7436 | 0.7870 | 0.8504 | 0.8848 | 0.9211 | 0.9400 | 0.9516 | 0.9595 | 0.9694 | 0.9754 |
| 1 | 0.1102 | 0.2306 | 0.3435 | 0.4388 | 0.5157 | 0.5770 | 0.6661 | 0.7259 | 0.7683 | 0.7995 | 0.8235 | 0.8576 | 0.9042 | 0.9278 | 0.9517 | 0.9637 | 0.9709 | 0.9758 | 0.9818 | 0.9854 |
| 2 | 0.1203 | 0.2618 | 0.3939 | 0.5009 | 0.5828 | 0.6448 | 0.7290 | 0.7820 | 0.8179 | 0.8437 | 0.8632 | 0.8904 | 0.9269 | 0.9451 | 0.9634 | 0.9725 | 0.9780 | 0.9817 | 0.9863 | 0.9890 |
| 3 | 0.1305 | 0.2920 | 0.4398 | 0.5534 | 0.6355 | 0.6945 | 0.7708 | 0.8170 | 0.8477 | 0.8695 | 0.8859 | 0.9088 | 0.9392 | 0.9544 | 0.9696 | 0.9772 | 0.9818 | 0.9848 | 0.9886 | 0.9909 |
| 4 | 0.1405 | 0.3212 | 0.4812 | 0.5973 | 0.6765 | 0.7312 | 0.7996 | 0.8403 | 0.8672 | 0.8863 | 0.9006 | 0.9205 | 0.9471 | 0.9603 | 0.9736 | 0.9802 | 0.9841 | 0.9868 | 0.9901 | 0.9921 |
| 5 | 0.1505 | 0.3491 | 0.5182 | 0.6335 | 0.7084 | 0.7586 | 0.8204 | 0.8569 | 0.8809 | 0.8981 | 0.9109 | 0.9288 | 0.9526 | 0.9644 | 0.9763 | 0.9822 | 0.9858 | 0.9882 | 0.9911 | 0.9929 |
| 6 | 0.1605 | 0.3758 | 0.5509 | 0.6635 | 0.7336 | 0.7798 | 0.8361 | 0.8693 | 0.8913 | 0.9069 | 0.9186 | 0.9349 | 0.9567 | 0.9675 | 0.9783 | 0.9838 | 0.9870 | 0.9892 | 0.9919 | 0.9935 |
| 7 | 0.1704 | 0.4012 | 0.5797 | 0.6883 | 0.7538 | 0.7965 | 0.8484 | 0.8790 | 0.8994 | 0.9138 | 0.9246 | 0.9397 | 0.9599 | 0.9699 | 0.9799 | 0.9850 | 0.9880 | 0.9900 | 0.9925 | 0.9940 |
| 8 | 0.1803 | 0.4251 | 0.6051 | 0.7090 | 0.7703 | 0.8099 | 0.8583 | 0.8869 | 0.9059 | 0.9194 | 0.9295 | 0.9436 | 0.9625 | 0.9718 | 0.9812 | 0.9859 | 0.9887 | 0.9906 | 0.9930 | 0.9944 |
| 9 | 0.1901 | 0.4478 | 0.6273 | 0.7265 | 0.7840 | 0.8211 | 0.8665 | 0.8934 | 0.9113 | 0.9240 | 0.9335 | 0.9469 | 0.9646 | 0.9735 | 0.9823 | 0.9867 | 0.9894 | 0.9912 | 0.9934 | 0.9947 |
| 10 | 0.1998 | 0.4690 | 0.6469 | 0.7413 | 0.7955 | 0.8305 | 0.8734 | 0.8989 | 0.9159 | 0.9279 | 0.9370 | 0.9496 | 0.9664 | 0.9748 | 0.9832 | 0.9874 | 0.9899 | 0.9916 | 0.9937 | 0.9950 |
| 11 | 0.2094 | 0.4890 | 0.6642 | 0.7541 | 0.8054 | 0.8386 | 0.8794 | 0.9037 | 0.9198 | 0.9313 | 0.9399 | 0.9519 | 0.9680 | 0.9760 | 0.9840 | 0.9880 | 0.9904 | 0.9920 | 0.9940 | 0.9952 |
| 12 | 0.2190 | 0.5077 | 0.6795 | 0.7652 | 0.8140 | 0.8456 | 0.8846 | 0.9078 | 0.9232 | 0.9342 | 0.9425 | 0.9540 | 0.9693 | 0.9770 | 0.9847 | 0.9885 | 0.9908 | 0.9923 | 0.9943 | 0.9954 |
| 13 | 0.2284 | 0.5251 | 0.6931 | 0.7750 | 0.8215 | 0.8518 | 0.8892 | 0.9114 | 0.9263 | 0.9368 | 0.9447 | 0.9558 | 0.9706 | 0.9779 | 0.9853 | 0.9890 | 0.9912 | 0.9926 | 0.9945 | 0.9956 |
| 14 | 0.2378 | 0.5414 | 0.7053 | 0.7836 | 0.8282 | 0.8573 | 0.8932 | 0.9147 | 0.9290 | 0.9391 | 0.9468 | 0.9574 | 0.9716 | 0.9787 | 0.9858 | 0.9894 | 0.9915 | 0.9929 | 0.9947 | 0.9957 |
| 15 | 0.2471 | 0.5567 | 0.7162 | 0.7913 | 0.8342 | 0.8622 | 0.8969 | 0.9176 | 0.9314 | 0.9412 | 0.9486 | 0.9589 | 0.9726 | 0.9794 | 0.9863 | 0.9897 | 0.9918 | 0.9932 | 0.9949 | 0.9959 |
| 16 | 0.2563 | 0.5709 | 0.7260 | 0.7983 | 0.8396 | 0.8666 | 0.9002 | 0.9202 | 0.9336 | 0.9431 | 0.9502 | 0.9602 | 0.9735 | 0.9801 | 0.9867 | 0.9901 | 0.9920 | 0.9934 | 0.9950 | 0.9960 |
| 17 | 0.2654 | 0.5842 | 0.7349 | 0.8045 | 0.8445 | 0.8707 | 0.9032 | 0.9226 | 0.9356 | 0.9448 | 0.9517 | 0.9614 | 0.9743 | 0.9807 | 0.9871 | 0.9903 | 0.9923 | 0.9936 | 0.9952 | 0.9961 |
| 18 | 0.2743 | 0.5966 | 0.7430 | 0.8103 | 0.8489 | 0.8744 | 0.9059 | 0.9248 | 0.9374 | 0.9463 | 0.9531 | 0.9625 | 0.9750 | 0.9812 | 0.9875 | 0.9906 | 0.9925 | 0.9937 | 0.9953 | 0.9962 |
| 19 | 0.2832 | 0.6081 | 0.7505 | 0.8155 | 0.8530 | 0.8777 | 0.9085 | 0.9268 | 0.9390 | 0.9478 | 0.9543 | 0.9635 | 0.9756 | 0.9817 | 0.9878 | 0.9909 | 0.9927 | 0.9939 | 0.9954 | 0.9963 |
| 20 | 0.2919 | 0.6189 | 0.7573 | 0.8203 | 0.8568 | 0.8809 | 0.9108 | 0.9287 | 0.9406 | 0.9491 | 0.9555 | 0.9644 | 0.9763 | 0.9822 | 0.9881 | 0.9911 | 0.9929 | 0.9941 | 0.9956 | 0.9964 |
| 21 | 0.3006 | 0.6291 | 0.7636 | 0.8248 | 0.8603 | 0.8838 | 0.9130 | 0.9304 | 0.9420 | 0.9503 | 0.9565 | 0.9652 | 0.9768 | 0.9826 | 0.9884 | 0.9913 | 0.9931 | 0.9942 | 0.9957 | 0.9965 |
| 22 | 0.3091 | 0.6385 | 0.7694 | 0.8289 | 0.8636 | 0.8865 | 0.9150 | 0.9320 | 0.9434 | 0.9515 | 0.9575 | 0.9660 | 0.9774 | 0.9830 | 0.9887 | 0.9915 | 0.9932 | 0.9943 | 0.9958 | 0.9966 |
| 23 | 0.3175 | 0.6474 | 0.7748 | 0.8328 | 0.8666 | 0.8890 | 0.9168 | 0.9335 | 0.9446 | 0.9525 | 0.9585 | 0.9668 | 0.9779 | 0.9834 | 0.9889 | 0.9917 | 0.9934 | 0.9945 | 0.9959 | 0.9967 |
| 24 | 0.3258 | 0.6558 | 0.7798 | 0.8364 | 0.8694 | 0.8913 | 0.9186 | 0.9349 | 0.9458 | 0.9535 | 0.9594 | 0.9675 | 0.9783 | 0.9838 | 0.9892 | 0.9919 | 0.9935 | 0.9946 | 0.9959 | 0.9968 |
| 25 | 0.3339 | 0.6636 | 0.7845 | 0.8397 | 0.8721 | 0.8936 | 0.9203 | 0.9362 | 0.9469 | 0.9545 | 0.9602 | 0.9681 | 0.9788 | 0.9841 | 0.9894 | 0.9920 | 0.9936 | 0.9947 | 0.9960 | 0.9968 |
| 26 | 0.3420 | 0.6710 | 0.7889 | 0.8429 | 0.8746 | 0.8956 | 0.9218 | 0.9375 | 0.9479 | 0.9554 | 0.9610 | 0.9688 | 0.9792 | 0.9844 | 0.9896 | 0.9922 | 0.9938 | 0.9948 | 0.9961 | 0.9969 |
| 27 | 0.3499 | 0.6780 | 0.7930 | 0.8459 | 0.8770 | 0.8976 | 0.9233 | 0.9387 | 0.9489 | 0.9562 | 0.9617 | 0.9694 | 0.9796 | 0.9847 | 0.9898 | 0.9923 | 0.9939 | 0.9949 | 0.9962 | 0.9969 |
| 28 | 0.3577 | 0.6845 | 0.7969 | 0.8487 | 0.8792 | 0.8995 | 0.9247 | 0.9398 | 0.9498 | 0.9570 | 0.9624 | 0.9699 | 0.9799 | 0.9850 | 0.9900 | 0.9925 | 0.9940 | 0.9950 | 0.9962 | 0.9970 |
| 29 | 0.3653 | 0.6907 | 0.8006 | 0.8514 | 0.8813 | 0.9012 | 0.9260 | 0.9408 | 0.9507 | 0.9577 | 0.9630 | 0.9704 | 0.9803 | 0.9852 | 0.9901 | 0.9926 | 0.9941 | 0.9951 | 0.9963 | 0.9970 |
| 30 | 0.3729 | 0.6966 | 0.8041 | 0.8539 | 0.8834 | 0.9029 | 0.9272 | 0.9418 | 0.9515 | 0.9585 | 0.9637 | 0.9709 | 0.9806 | 0.9855 | 0.9903 | 0.9927 | 0.9942 | 0.9952 | 0.9964 | 0.9971 |
| 31 | 0.3803 | 0.7022 | 0.8074 | 0.8563 | 0.8853 | 0.9045 | 0.9284 | 0.9428 | 0.9523 | 0.9591 | 0.9642 | 0.9714 | 0.9809 | 0.9857 | 0.9905 | 0.9929 | 0.9943 | 0.9952 | 0.9964 | 0.9971 |

| | | | | | | | | | | | | | | | | | | | | |
|---|---|---|---|---|---|---|---|---|---|---|---|---|---|---|---|---|---|---|---|---|
| **32** | 0.3876 | 0.7074 | 0.8106 | 0.8586 | 0.8871 | 0.9060 | 0.9296 | 0.9437 | 0.9531 | 0.9598 | 0.9648 | 0.9719 | 0.9812 | 0.9859 | 0.9906 | 0.9930 | 0.9944 | 0.9953 | 0.9965 | 0.9972 |
| **33** | 0.3947 | 0.7124 | 0.8135 | 0.8608 | 0.8888 | 0.9074 | 0.9306 | 0.9445 | 0.9538 | 0.9604 | 0.9653 | 0.9723 | 0.9815 | 0.9861 | 0.9908 | 0.9931 | 0.9945 | 0.9954 | 0.9965 | 0.9972 |
| **34** | 0.4018 | 0.7172 | 0.8164 | 0.8629 | 0.8905 | 0.9088 | 0.9317 | 0.9454 | 0.9545 | 0.9610 | 0.9659 | 0.9727 | 0.9818 | 0.9863 | 0.9909 | 0.9932 | 0.9945 | 0.9955 | 0.9966 | 0.9973 |
| **35** | 0.4087 | 0.7218 | 0.8191 | 0.8649 | 0.8921 | 0.9101 | 0.9326 | 0.9461 | 0.9551 | 0.9615 | 0.9664 | 0.9731 | 0.9821 | 0.9865 | 0.9910 | 0.9933 | 0.9946 | 0.9955 | 0.9966 | 0.9973 |
| **36** | 0.4155 | 0.7261 | 0.8217 | 0.8668 | 0.8936 | 0.9114 | 0.9336 | 0.9469 | 0.9558 | 0.9621 | 0.9668 | 0.9735 | 0.9823 | 0.9867 | 0.9912 | 0.9934 | 0.9947 | 0.9956 | 0.9967 | 0.9973 |
| **37** | 0.4221 | 0.7302 | 0.8242 | 0.8686 | 0.8951 | 0.9126 | 0.9345 | 0.9476 | 0.9564 | 0.9626 | 0.9673 | 0.9738 | 0.9826 | 0.9869 | 0.9913 | 0.9935 | 0.9948 | 0.9956 | 0.9967 | 0.9974 |
| **38** | 0.4287 | 0.7342 | 0.8266 | 0.8704 | 0.8965 | 0.9138 | 0.9354 | 0.9483 | 0.9569 | 0.9631 | 0.9677 | 0.9742 | 0.9828 | 0.9871 | 0.9914 | 0.9935 | 0.9948 | 0.9957 | 0.9968 | 0.9974 |
| **39** | 0.4351 | 0.7380 | 0.8289 | 0.8721 | 0.8978 | 0.9149 | 0.9362 | 0.9490 | 0.9575 | 0.9636 | 0.9681 | 0.9745 | 0.9830 | 0.9873 | 0.9915 | 0.9936 | 0.9949 | 0.9958 | 0.9968 | 0.9975 |
| **40** | 0.4414 | 0.7416 | 0.8311 | 0.8737 | 0.8991 | 0.9160 | 0.9370 | 0.9496 | 0.9580 | 0.9640 | 0.9685 | 0.9748 | 0.9832 | 0.9874 | 0.9916 | 0.9937 | 0.9950 | 0.9958 | 0.9969 | 0.9975 |
| **41** | 0.4476 | 0.7451 | 0.8332 | 0.8753 | 0.9003 | 0.9170 | 0.9378 | 0.9502 | 0.9585 | 0.9645 | 0.9689 | 0.9751 | 0.9834 | 0.9876 | 0.9917 | 0.9938 | 0.9950 | 0.9959 | 0.9969 | 0.9975 |
| **42** | 0.4537 | 0.7484 | 0.8352 | 0.8768 | 0.9015 | 0.9180 | 0.9385 | 0.9508 | 0.9590 | 0.9649 | 0.9693 | 0.9754 | 0.9836 | 0.9877 | 0.9918 | 0.9939 | 0.9951 | 0.9959 | 0.9969 | 0.9975 |
| **43** | 0.4596 | 0.7516 | 0.8372 | 0.8782 | 0.9027 | 0.9190 | 0.9393 | 0.9514 | 0.9595 | 0.9653 | 0.9696 | 0.9757 | 0.9838 | 0.9879 | 0.9919 | 0.9939 | 0.9951 | 0.9960 | 0.9970 | 0.9976 |
| **44** | 0.4654 | 0.7547 | 0.8391 | 0.8796 | 0.9038 | 0.9199 | 0.9399 | 0.9520 | 0.9600 | 0.9657 | 0.9700 | 0.9760 | 0.9840 | 0.9880 | 0.9920 | 0.9940 | 0.9952 | 0.9960 | 0.9970 | 0.9976 |
| **45** | 0.4712 | 0.7577 | 0.8409 | 0.8810 | 0.9049 | 0.9208 | 0.9406 | 0.9525 | 0.9604 | 0.9661 | 0.9703 | 0.9763 | 0.9842 | 0.9881 | 0.9921 | 0.9941 | 0.9953 | 0.9960 | 0.9970 | 0.9976 |
| **46** | 0.4768 | 0.7605 | 0.8427 | 0.8823 | 0.9059 | 0.9217 | 0.9413 | 0.9530 | 0.9609 | 0.9665 | 0.9707 | 0.9765 | 0.9844 | 0.9883 | 0.9922 | 0.9941 | 0.9953 | 0.9961 | 0.9971 | 0.9977 |
| **47** | 0.4823 | 0.7633 | 0.8444 | 0.8836 | 0.9069 | 0.9225 | 0.9419 | 0.9535 | 0.9613 | 0.9668 | 0.9710 | 0.9768 | 0.9845 | 0.9884 | 0.9923 | 0.9942 | 0.9954 | 0.9961 | 0.9971 | 0.9977 |
| **48** | 0.4877 | 0.7660 | 0.8461 | 0.8848 | 0.9079 | 0.9233 | 0.9425 | 0.9540 | 0.9617 | 0.9672 | 0.9713 | 0.9770 | 0.9847 | 0.9885 | 0.9923 | 0.9943 | 0.9954 | 0.9962 | 0.9971 | 0.9977 |
| **49** | 0.4929 | 0.7685 | 0.8477 | 0.8860 | 0.9089 | 0.9241 | 0.9431 | 0.9545 | 0.9621 | 0.9675 | 0.9716 | 0.9773 | 0.9848 | 0.9886 | 0.9924 | 0.9943 | 0.9955 | 0.9962 | 0.9972 | 0.9977 |
| **50** | 0.4981 | 0.7710 | 0.8492 | 0.8871 | 0.9098 | 0.9249 | 0.9437 | 0.9550 | 0.9625 | 0.9678 | 0.9719 | 0.9775 | 0.9850 | 0.9887 | 0.9925 | 0.9944 | 0.9955 | 0.9962 | 0.9972 | 0.9977 |
| **51** | 0.5032 | 0.7734 | 0.8507 | 0.8883 | 0.9107 | 0.9256 | 0.9442 | 0.9554 | 0.9628 | 0.9681 | 0.9721 | 0.9777 | 0.9851 | 0.9889 | 0.9926 | 0.9944 | 0.9955 | 0.9963 | 0.9972 | 0.9978 |
| **52** | 0.5082 | 0.7758 | 0.8522 | 0.8894 | 0.9116 | 0.9263 | 0.9448 | 0.9558 | 0.9632 | 0.9685 | 0.9724 | 0.9779 | 0.9853 | 0.9890 | 0.9926 | 0.9945 | 0.9956 | 0.9963 | 0.9972 | 0.9978 |
| **53** | 0.5131 | 0.7780 | 0.8536 | 0.8904 | 0.9124 | 0.9270 | 0.9453 | 0.9562 | 0.9635 | 0.9688 | 0.9727 | 0.9781 | 0.9854 | 0.9891 | 0.9927 | 0.9945 | 0.9956 | 0.9964 | 0.9973 | 0.9978 |
| **54** | 0.5179 | 0.7802 | 0.8550 | 0.8914 | 0.9132 | 0.9277 | 0.9458 | 0.9567 | 0.9639 | 0.9690 | 0.9729 | 0.9783 | 0.9856 | 0.9892 | 0.9928 | 0.9946 | 0.9957 | 0.9964 | 0.9973 | 0.9978 |
| **55** | 0.5225 | 0.7823 | 0.8563 | 0.8924 | 0.9140 | 0.9284 | 0.9463 | 0.9571 | 0.9642 | 0.9693 | 0.9732 | 0.9785 | 0.9857 | 0.9893 | 0.9928 | 0.9946 | 0.9957 | 0.9964 | 0.9973 | 0.9979 |
| **56** | 0.5271 | 0.7844 | 0.8576 | 0.8934 | 0.9148 | 0.9290 | 0.9468 | 0.9574 | 0.9645 | 0.9696 | 0.9734 | 0.9787 | 0.9858 | 0.9894 | 0.9929 | 0.9947 | 0.9957 | 0.9965 | 0.9973 | 0.9979 |
| **57** | 0.5316 | 0.7864 | 0.8589 | 0.8943 | 0.9155 | 0.9296 | 0.9473 | 0.9578 | 0.9648 | 0.9699 | 0.9736 | 0.9789 | 0.9859 | 0.9895 | 0.9930 | 0.9947 | 0.9958 | 0.9965 | 0.9974 | 0.9979 |
| **58** | 0.5361 | 0.7883 | 0.8601 | 0.8953 | 0.9163 | 0.9303 | 0.9477 | 0.9582 | 0.9652 | 0.9701 | 0.9739 | 0.9791 | 0.9861 | 0.9895 | 0.9930 | 0.9948 | 0.9958 | 0.9965 | 0.9974 | 0.9979 |
| **59** | 0.5404 | 0.7902 | 0.8613 | 0.8962 | 0.9170 | 0.9308 | 0.9482 | 0.9585 | 0.9655 | 0.9704 | 0.9741 | 0.9793 | 0.9862 | 0.9896 | 0.9931 | 0.9948 | 0.9959 | 0.9965 | 0.9974 | 0.9979 |
| **60** | 0.5446 | 0.7921 | 0.8625 | 0.8970 | 0.9177 | 0.9314 | 0.9486 | 0.9589 | 0.9657 | 0.9706 | 0.9743 | 0.9794 | 0.9863 | 0.9897 | 0.9932 | 0.9949 | 0.9959 | 0.9966 | 0.9974 | 0.9979 |
| **61** | 0.5488 | 0.7939 | 0.8636 | 0.8979 | 0.9184 | 0.9320 | 0.9490 | 0.9592 | 0.9660 | 0.9709 | 0.9745 | 0.9796 | 0.9864 | 0.9898 | 0.9932 | 0.9949 | 0.9959 | 0.9966 | 0.9975 | 0.9980 |
| **62** | 0.5528 | 0.7956 | 0.8648 | 0.8987 | 0.9190 | 0.9325 | 0.9494 | 0.9596 | 0.9663 | 0.9711 | 0.9747 | 0.9798 | 0.9865 | 0.9899 | 0.9933 | 0.9949 | 0.9960 | 0.9966 | 0.9975 | 0.9980 |
| **63** | 0.5568 | 0.7973 | 0.8658 | 0.8995 | 0.9197 | 0.9331 | 0.9498 | 0.9599 | 0.9666 | 0.9713 | 0.9749 | 0.9799 | 0.9866 | 0.9900 | 0.9933 | 0.9950 | 0.9960 | 0.9967 | 0.9975 | 0.9980 |
| **64** | 0.5608 | 0.7990 | 0.8669 | 0.9003 | 0.9203 | 0.9336 | 0.9502 | 0.9602 | 0.9668 | 0.9716 | 0.9751 | 0.9801 | 0.9867 | 0.9901 | 0.9934 | 0.9950 | 0.9960 | 0.9967 | 0.9975 | 0.9980 |
| **65** | 0.5646 | 0.8006 | 0.8679 | 0.9011 | 0.9209 | 0.9341 | 0.9506 | 0.9605 | 0.9671 | 0.9718 | 0.9753 | 0.9803 | 0.9868 | 0.9901 | 0.9934 | 0.9951 | 0.9961 | 0.9967 | 0.9975 | 0.9980 |
| **66** | 0.5684 | 0.8021 | 0.8690 | 0.9018 | 0.9215 | 0.9346 | 0.9510 | 0.9608 | 0.9673 | 0.9720 | 0.9755 | 0.9804 | 0.9869 | 0.9902 | 0.9935 | 0.9951 | 0.9961 | 0.9967 | 0.9976 | 0.9980 |
| **67** | 0.5720 | 0.8037 | 0.8699 | 0.9026 | 0.9221 | 0.9351 | 0.9514 | 0.9611 | 0.9676 | 0.9722 | 0.9757 | 0.9806 | 0.9870 | 0.9903 | 0.9935 | 0.9951 | 0.9961 | 0.9968 | 0.9976 | 0.9981 |
| **68** | 0.5757 | 0.8052 | 0.8709 | 0.9033 | 0.9227 | 0.9356 | 0.9517 | 0.9614 | 0.9678 | 0.9724 | 0.9759 | 0.9807 | 0.9871 | 0.9903 | 0.9936 | 0.9952 | 0.9961 | 0.9968 | 0.9976 | 0.9981 |

| | | | | | | | | | | | | | | | | | | | | |
|---|---|---|---|---|---|---|---|---|---|---|---|---|---|---|---|---|---|---|---|---|
| **69** | 0.5792 | 0.8067 | 0.8719 | 0.9040 | 0.9233 | 0.9361 | 0.9521 | 0.9617 | 0.9681 | 0.9726 | 0.9760 | 0.9808 | 0.9872 | 0.9904 | 0.9936 | 0.9952 | 0.9962 | 0.9968 | 0.9976 | 0.9981 |
| **70** | 0.5827 | 0.8081 | 0.8728 | 0.9047 | 0.9238 | 0.9365 | 0.9524 | 0.9619 | 0.9683 | 0.9728 | 0.9762 | 0.9810 | 0.9873 | 0.9905 | 0.9937 | 0.9952 | 0.9962 | 0.9968 | 0.9976 | 0.9981 |
| **71** | 0.5861 | 0.8095 | 0.8737 | 0.9054 | 0.9243 | 0.9370 | 0.9527 | 0.9622 | 0.9685 | 0.9730 | 0.9764 | 0.9811 | 0.9874 | 0.9906 | 0.9937 | 0.9953 | 0.9962 | 0.9969 | 0.9976 | 0.9981 |
| **72** | 0.5894 | 0.8109 | 0.8746 | 0.9060 | 0.9249 | 0.9374 | 0.9531 | 0.9625 | 0.9687 | 0.9732 | 0.9765 | 0.9812 | 0.9875 | 0.9906 | 0.9937 | 0.9953 | 0.9962 | 0.9969 | 0.9977 | 0.9981 |
| **73** | 0.5927 | 0.8122 | 0.8754 | 0.9067 | 0.9254 | 0.9378 | 0.9534 | 0.9627 | 0.9689 | 0.9734 | 0.9767 | 0.9814 | 0.9876 | 0.9907 | 0.9938 | 0.9953 | 0.9963 | 0.9969 | 0.9977 | 0.9981 |
| **74** | 0.5959 | 0.8135 | 0.8763 | 0.9073 | 0.9259 | 0.9383 | 0.9537 | 0.9630 | 0.9692 | 0.9736 | 0.9769 | 0.9815 | 0.9877 | 0.9907 | 0.9938 | 0.9954 | 0.9963 | 0.9969 | 0.9977 | 0.9981 |
| **75** | 0.5991 | 0.8148 | 0.8771 | 0.9080 | 0.9264 | 0.9387 | 0.9540 | 0.9632 | 0.9694 | 0.9737 | 0.9770 | 0.9816 | 0.9877 | 0.9908 | 0.9939 | 0.9954 | 0.9963 | 0.9969 | 0.9977 | 0.9982 |
| **76** | 0.6022 | 0.8161 | 0.8779 | 0.9086 | 0.9269 | 0.9391 | 0.9543 | 0.9635 | 0.9696 | 0.9739 | 0.9772 | 0.9817 | 0.9878 | 0.9909 | 0.9939 | 0.9954 | 0.9963 | 0.9970 | 0.9977 | 0.9982 |
| **77** | 0.6052 | 0.8173 | 0.8787 | 0.9092 | 0.9274 | 0.9395 | 0.9546 | 0.9637 | 0.9698 | 0.9741 | 0.9773 | 0.9819 | 0.9879 | 0.9909 | 0.9940 | 0.9955 | 0.9964 | 0.9970 | 0.9977 | 0.9982 |
| **78** | 0.6082 | 0.8185 | 0.8795 | 0.9097 | 0.9278 | 0.9399 | 0.9549 | 0.9639 | 0.9700 | 0.9742 | 0.9775 | 0.9820 | 0.9880 | 0.9910 | 0.9940 | 0.9955 | 0.9964 | 0.9970 | 0.9977 | 0.9982 |
| **79** | 0.6111 | 0.8197 | 0.8803 | 0.9103 | 0.9283 | 0.9403 | 0.9552 | 0.9642 | 0.9701 | 0.9744 | 0.9776 | 0.9821 | 0.9881 | 0.9910 | 0.9940 | 0.9955 | 0.9964 | 0.9970 | 0.9978 | 0.9982 |
| **80** | 0.6140 | 0.8208 | 0.8811 | 0.9109 | 0.9287 | 0.9406 | 0.9555 | 0.9644 | 0.9703 | 0.9746 | 0.9778 | 0.9822 | 0.9881 | 0.9911 | 0.9941 | 0.9956 | 0.9964 | 0.9970 | 0.9978 | 0.9982 |
| **81** | 0.6168 | 0.8220 | 0.8818 | 0.9114 | 0.9292 | 0.9410 | 0.9558 | 0.9646 | 0.9705 | 0.9747 | 0.9779 | 0.9823 | 0.9882 | 0.9912 | 0.9941 | 0.9956 | 0.9965 | 0.9971 | 0.9978 | 0.9982 |
| **82** | 0.6196 | 0.8231 | 0.8825 | 0.9120 | 0.9296 | 0.9414 | 0.9560 | 0.9648 | 0.9707 | 0.9749 | 0.9780 | 0.9824 | 0.9883 | 0.9912 | 0.9941 | 0.9956 | 0.9965 | 0.9971 | 0.9978 | 0.9982 |
| **83** | 0.6223 | 0.8242 | 0.8832 | 0.9125 | 0.9300 | 0.9417 | 0.9563 | 0.9650 | 0.9709 | 0.9750 | 0.9782 | 0.9825 | 0.9884 | 0.9913 | 0.9942 | 0.9956 | 0.9965 | 0.9971 | 0.9978 | 0.9983 |
| **84** | 0.6250 | 0.8252 | 0.8839 | 0.9130 | 0.9305 | 0.9421 | 0.9566 | 0.9653 | 0.9710 | 0.9752 | 0.9783 | 0.9826 | 0.9884 | 0.9913 | 0.9942 | 0.9957 | 0.9965 | 0.9971 | 0.9978 | 0.9983 |
| **85** | 0.6276 | 0.8263 | 0.8846 | 0.9136 | 0.9309 | 0.9424 | 0.9568 | 0.9655 | 0.9712 | 0.9753 | 0.9784 | 0.9827 | 0.9885 | 0.9914 | 0.9942 | 0.9957 | 0.9965 | 0.9971 | 0.9978 | 0.9983 |
| **86** | 0.6302 | 0.8273 | 0.8853 | 0.9141 | 0.9313 | 0.9427 | 0.9571 | 0.9657 | 0.9714 | 0.9755 | 0.9785 | 0.9828 | 0.9886 | 0.9914 | 0.9943 | 0.9957 | 0.9966 | 0.9971 | 0.9979 | 0.9983 |
| **87** | 0.6327 | 0.8284 | 0.8860 | 0.9146 | 0.9317 | 0.9431 | 0.9573 | 0.9659 | 0.9716 | 0.9756 | 0.9787 | 0.9829 | 0.9886 | 0.9915 | 0.9943 | 0.9957 | 0.9966 | 0.9972 | 0.9979 | 0.9983 |
| **88** | 0.6352 | 0.8293 | 0.8866 | 0.9150 | 0.9321 | 0.9434 | 0.9576 | 0.9661 | 0.9717 | 0.9758 | 0.9788 | 0.9830 | 0.9887 | 0.9915 | 0.9943 | 0.9958 | 0.9966 | 0.9972 | 0.9979 | 0.9983 |
| **89** | 0.6376 | 0.8303 | 0.8873 | 0.9155 | 0.9325 | 0.9437 | 0.9578 | 0.9662 | 0.9719 | 0.9759 | 0.9789 | 0.9831 | 0.9888 | 0.9916 | 0.9944 | 0.9958 | 0.9966 | 0.9972 | 0.9979 | 0.9983 |
| **90** | 0.6400 | 0.8313 | 0.8879 | 0.9160 | 0.9328 | 0.9440 | 0.9580 | 0.9664 | 0.9720 | 0.9760 | 0.9790 | 0.9832 | 0.9888 | 0.9916 | 0.9944 | 0.9958 | 0.9966 | 0.9972 | 0.9979 | 0.9983 |
| **91** | 0.6423 | 0.8322 | 0.8885 | 0.9165 | 0.9332 | 0.9443 | 0.9583 | 0.9666 | 0.9722 | 0.9762 | 0.9791 | 0.9833 | 0.9889 | 0.9917 | 0.9944 | 0.9958 | 0.9967 | 0.9972 | 0.9979 | 0.9983 |
| **92** | 0.6446 | 0.8332 | 0.8891 | 0.9169 | 0.9336 | 0.9446 | 0.9585 | 0.9668 | 0.9723 | 0.9763 | 0.9793 | 0.9834 | 0.9889 | 0.9917 | 0.9945 | 0.9959 | 0.9967 | 0.9972 | 0.9979 | 0.9983 |
| **93** | 0.6469 | 0.8341 | 0.8897 | 0.9174 | 0.9339 | 0.9449 | 0.9587 | 0.9670 | 0.9725 | 0.9764 | 0.9794 | 0.9835 | 0.9890 | 0.9917 | 0.9945 | 0.9959 | 0.9967 | 0.9972 | 0.9979 | 0.9983 |
| **94** | 0.6492 | 0.8350 | 0.8903 | 0.9178 | 0.9343 | 0.9452 | 0.9589 | 0.9672 | 0.9726 | 0.9765 | 0.9795 | 0.9836 | 0.9891 | 0.9918 | 0.9945 | 0.9959 | 0.9967 | 0.9973 | 0.9979 | 0.9984 |
| **95** | 0.6513 | 0.8359 | 0.8909 | 0.9182 | 0.9346 | 0.9455 | 0.9592 | 0.9673 | 0.9728 | 0.9767 | 0.9796 | 0.9837 | 0.9891 | 0.9918 | 0.9946 | 0.9959 | 0.9967 | 0.9973 | 0.9980 | 0.9984 |
| **96** | 0.6535 | 0.8367 | 0.8915 | 0.9187 | 0.9350 | 0.9458 | 0.9594 | 0.9675 | 0.9729 | 0.9768 | 0.9797 | 0.9838 | 0.9892 | 0.9919 | 0.9946 | 0.9959 | 0.9968 | 0.9973 | 0.9980 | 0.9984 |
| **97** | 0.6556 | 0.8376 | 0.8920 | 0.9191 | 0.9353 | 0.9461 | 0.9596 | 0.9677 | 0.9731 | 0.9769 | 0.9798 | 0.9838 | 0.9892 | 0.9919 | 0.9946 | 0.9960 | 0.9968 | 0.9973 | 0.9980 | 0.9984 |
| **98** | 0.6577 | 0.8384 | 0.8926 | 0.9195 | 0.9356 | 0.9464 | 0.9598 | 0.9678 | 0.9732 | 0.9770 | 0.9799 | 0.9839 | 0.9893 | 0.9920 | 0.9946 | 0.9960 | 0.9968 | 0.9973 | 0.9980 | 0.9984 |
| **99** | 0.6598 | 0.8393 | 0.8931 | 0.9199 | 0.9360 | 0.9466 | 0.9600 | 0.9680 | 0.9733 | 0.9771 | 0.9800 | 0.9840 | 0.9893 | 0.9920 | 0.9947 | 0.9960 | 0.9968 | 0.9973 | 0.9980 | 0.9984 |
| **100** | 0.6618 | 0.8401 | 0.8937 | 0.9203 | 0.9363 | 0.9469 | 0.9602 | 0.9682 | 0.9735 | 0.9773 | 0.9801 | 0.9841 | 0.9894 | 0.9920 | 0.9947 | 0.9960 | 0.9968 | 0.9973 | 0.9980 | 0.9984 |
